# Supplementary material for: Predissociation of methyl cyanoformate: The HCN and HNC channels
Source: arXiv:1606.06230 ancillary file (2017-10-06)
Supplement: Supplementary file 1 [file Supplementary_Information.pdf]

# Photolytic production of HCN and HNC in astrophysical environments: A study of methyl cyanoformate

Michael J. Wilhelm[1,*], Emilio Martínez-Núñez[2,*], Jesús González-Vázquez[3], Saulo A. Vázquez[2], Jonathan M. Smith[1], and Hai-Lung Dai[1]

*1. Department of Chemistry, Temple University, 1901 N. 13th Street, Philadelphia, Pennsylvania 19102, USA.*
*2. Departamento de Química Física, Campus Vida, Universidade de Santiago de Compostela, 15782, Santiago de Compostela, Spain.*
*3. Departamento de Química, Universidad Autónoma de Madrid, Módulo 13, 28049 Madrid, Spain.*
*Authors to whom correspondence should be addressed: michael.wilhelm@temple.edu; emilio.nunez@usc.es

# Supplementary Information

## Index:


| | |
|---|---|
| **Excited state calculations** | 3 |
| **TSSCDS Calculations** | 13 |
| List of minima | 16 |
| List of transition states | 30 |
| **Kinetic calculations** | 65 |
| Preliminary KMC simulation | 65 |
| Second KMC simulation | 67 |
| **QCT Simulations** | 70 |
| PM3-SRP | 70 |
| QCT Details | 76 |
| **References** | 79 |

# Excited state calculations

The active space orbitals corresponding to ground state equilibrium geometry optimized at the SA-5-CASSCF/cc-pVTZ level are depicted in Figure 1S.

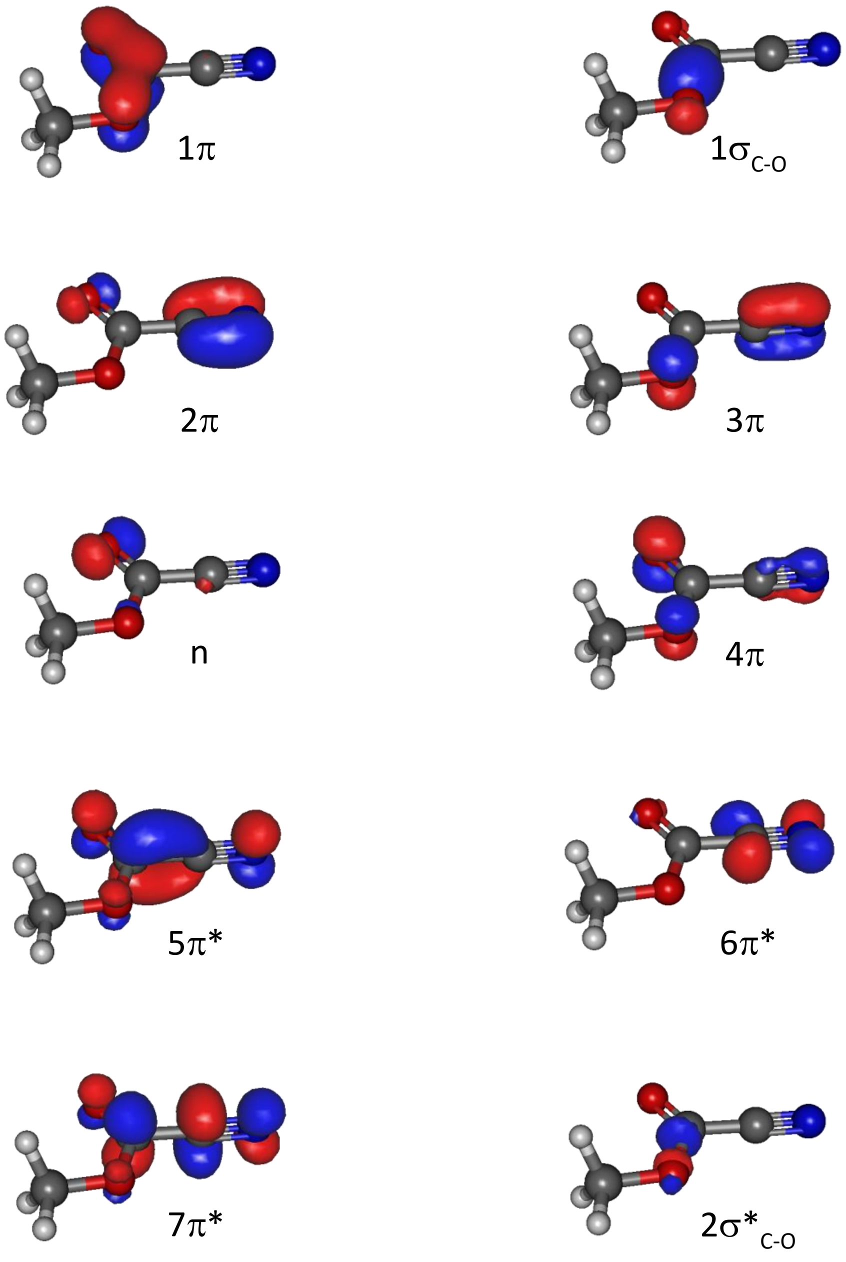


**Figure 1S.** Molecular orbitals comprising the active space.

Information about the nature of the calculated excited states is shown in Table 1S and in Figure 2S. The table presents the main configuration interaction coefficients for the low-lying valence excited states obtained at the MS-CASPT2 level and using the geometry optimized by SA-5-CASSCF/cc-pVTZ calculations. The figure depicts the CASSCF changes in the electron densities occurring upon transition from the electronic ground state.

**Table 1S:** Main MS-CASPT2 configuration interaction coefficients for the S1-S4 excited states of methyl cyanoformate.

| State symmetry | Main Configurations |
|---|---|
| $1^1A''$ ($S_1$) | n→5π* (−0.70), 2π→5π* (−0.56) |
| $1^1A'$ ($S_2$) | 4π→5π* (0.73), 3π→5π* (0.45) |
| $2^1A''$ ($S_3$) | 2π→5π* (0.71), n→5π* (−0.53) |
| $2^1A'$ ($S_4$) | 3π→5π* (0.68), 2π→6π* (0.49) |

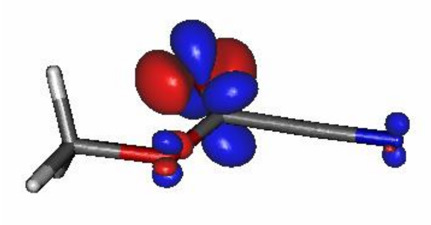

$S_1 - S_0$

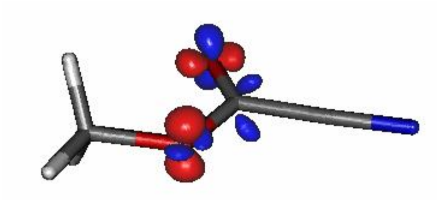

$S_2 - S_0$

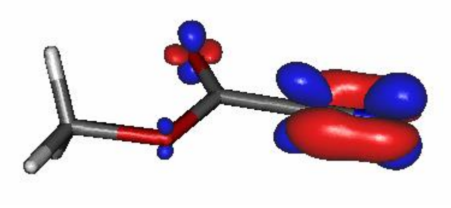

$S_3 - S_0$

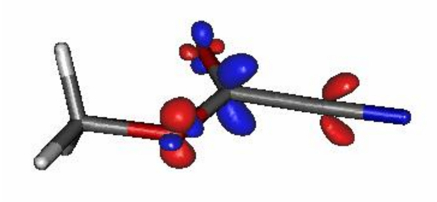

$S_4 - S_0$

**Figure 2S.** Electron density differences between the excited states and the electronic ground state calculated at the SA-5-CASSCF level. The transitions lead to electron transfer from regions in red to regions in blue.

The following geometries (Cartesian coordinates in Å) are the equilibrium structures for the lowest lying singlet states, obtained by SA-5-CASSCF/cc-pVTZ, as well as for the minimum energy crossing point (MECP) between the S2 and S3 surfaces. The MS-5-CASPT2 energies (in a.u.) are also indicated. For the equilibrium structure corresponding to the S3 state and for the MECP, the optimizations were performed under $C_S$ symmetry. The remaining optimizations were conducted without symmetry constraints.

**S0**

-320.73648850

| | | | |
|---|---|---|---|
| H1 | -2.5376284732 | -1.3170190049 | -0.0004512077 |
| H2 | -2.3213235990 | 0.2021283432 | 0.8829762962 |
| H3 | -2.3209989581 | 0.2031331003 | -0.8820286572 |
| C1 | -2.0521186913 | -0.3562738842 | 0.0002022059 |
| C2 | 0.1548670124 | 0.4349180571 | -0.0000122027 |
| C3 | 1.5536742090 | 0.0156956596 | 0.0000743390 |
| N | 2.6663495208 | -0.2848882196 | 0.0001192869 |
| O1 | -0.6558442836 | -0.6344409707 | 0.0003202795 |
| O2 | -0.1681567371 | 1.5725099193 | 0.0001596602 |

**S1**

-320.57861972

| | | | |
|---|---|---|---|
| H1 | -2.6184269116 | -1.2669338368 | 0.0005795113 |
| H2 | -2.3128433918 | 0.2262035318 | 0.8862395927 |
| H3 | -2.3134294151 | 0.2254478712 | -0.8867199402 |
| C1 | -2.0676044016 | -0.3420677679 | -0.0000757707 |
| C2 | 0.2276368196 | 0.2721942491 | 0.0002112448 |
| C3 | 1.5788735493 | 0.0352225737 | 0.0000004259 |
| N | 2.7335418107 | -0.1619402629 | -0.0001769301 |
| O1 | -0.7002339057 | -0.7174534760 | -0.0004204250 |
| O2 | -0.2086941539 | 1.5650901178 | 0.0017222912 |

**S3**

-320.50302241

| | | | |
|---|---|---|---|
| H1 | -2.5956355650 | -1.2909964416 | 0.0000000000 |
| H2 | -2.3267881079 | 0.2163105871 | 0.8820143051 |
| H3 | -2.3267881079 | 0.2163105871 | -0.8820143051 |
| C1 | -2.0683780575 | -0.3514313780 | 0.0000000000 |
| C2 | 0.1665964011 | 0.3768100422 | 0.0000000000 |
| C3 | 1.5080404089 | 0.0116927887 | 0.0000000000 |
| N | 2.7655114931 | -0.2042286389 | 0.0000000000 |
| O1 | -0.6933245248 | -0.6891199929 | 0.0000000000 |
| O2 | -0.1501215530 | 1.5539783583 | 0.0000000000 |

**S4**

-320.49595475

| | | | |
|---|---|---|---|
| H1 | -2.6217761966 | -1.2829479596 | -0.0002660125 |
| H2 | -2.3079106193 | 0.2238355426 | 0.8811327769 |
| H3 | -2.3078188232 | 0.2244822377 | -0.8805582294 |
| C1 | -2.0724540899 | -0.3566953059 | 0.0000863695 |
| C2 | 0.2041677967 | 0.3723872906 | 0.0007945036 |
| C3 | 1.5199471232 | -0.0310933742 | 0.0003013190 |
| N | 2.7662638755 | -0.1394571676 | -0.0002976671 |
| O1 | -0.7070529956 | -0.7144367545 | 0.0000298627 |
| O2 | -0.1545460707 | 1.5396884909 | 0.0001370772 |

**MECP**

-320.50302241 (S2) -320.49630483 (S3)

| | | | |
|---|---|---|---|
| H | -2.5956355650 | -1.2909964416 | 0.0000000000 |
| H | -2.3267881079 | 0.2163105871 | 0.8820143051 |
| H | -2.3267881079 | 0.2163105871 | -0.8820143051 |
| C | -2.0683780575 | -0.3514313780 | 0.0000000000 |
| C | 0.1665964011 | 0.3768100422 | 0.0000000000 |
| C | 1.5080404089 | 0.0116927887 | 0.0000000000 |
| N | 2.7655114931 | -0.2042286389 | 0.0000000000 |
| O | -0.6933245248 | -0.6891199929 | 0.0000000000 |
| O | -0.1501215530 | 1.5539783583 | 0.0000000000 |

Below are the ground state geometries (Cartesian coordinates in Å) optimized at the SA-5-CASSCF/cc-pVTZ level, constraining the O-C distance, and the corresponding MS-CASPT2 energies (in a.u.).

**C-O distance = 1.14 Å**

-320.69347619 -320.48999307 -320.42058140 -320.42055946 -320.37479291

| | | | |
|---|---|---|---|
| H1 | -2.5557712269 | -0.2385425243 | 0.8872345531 |
| H2 | -2.5575373064 | -1.7788404358 | -0.0035039133 |
| H3 | -2.5537341084 | -0.2297298594 | -0.8794339638 |
| C1 | 1.2949192001 | -0.1040709218 | -0.0011303699 |
| C2 | -0.1724685133 | 0.1377452358 | -0.0025030400 |
| C3 | -2.2279359943 | -0.7561820102 | 0.0016351177 |
| N | 2.4383932912 | -0.2767161655 | 0.0055101202 |
| O1 | -0.5417493491 | 1.2785757406 | -0.0089858513 |
| O2 | -0.7931109928 | -0.8184810595 | 0.0033523472 |

**C-O distance = 1.24 Å**

-320.72940391 -320.52894890 -320.46532437 -320.45872980 -320.44959202

| | | | |
|---|---|---|---|
| H1 | -2.5000217851 | -1.3203526054 | -0.0020036309 |
| H2 | -2.3180540020 | 0.2066232030 | 0.8832803224 |
| H3 | -2.3204021912 | 0.2098837437 | -0.8821834633 |
| C1 | -2.0452080417 | -0.3458351938 | -0.0008372623 |
| C2 | 0.1213230577 | 0.3992711062 | 0.0011083534 |
| C3 | 1.5381169868 | 0.0027360392 | -0.0000736326 |
| N | 2.6538742849 | -0.2863000871 | -0.0009159018 |
| O1 | -0.6356665504 | -0.5828435212 | -0.0030859309 |
| O2 | -0.1751417591 | 1.5525803155 | 0.0060711460 |

**C-O distance = 1.34 Å**

-320.73652852 -320.54057254 -320.48267315 -320.47193773 -320.46515484

| | | | |
|---|---|---|---|
| H1 | -2.5560532921 | -0.2451435160 | 0.8844653913 |
| H2 | -2.6297431803 | -1.7765597083 | -0.0012052729 |
| H3 | -2.5543708552 | -0.2416283915 | -0.8806146085 |
| C1 | 1.3204098164 | -0.0755928133 | -0.0007423464 |
| C2 | -0.1111532579 | 0.2152533803 | -0.0013114487 |
| C3 | -2.2356862217 | -0.7748740358 | 0.0011543756 |
| N | 2.4538726931 | -0.2842163480 | 0.0042528297 |
| O1 | -0.5368529160 | 1.3187840981 | -0.0062611963 |
| O2 | -0.8194177863 | -0.9222646656 | 0.0024372762 |

**C-O distance = 1.44 Å**

-320.72938564 -320.53810593 -320.49603006 -320.47122290 -320.46268143

| | | | |
|---|---|---|---|
| H1 | -2.5728189221 | -1.3149011694 | 0.0010711680 |

| | | | |
|---|---|---|---|
| H2 | -2.3231289734 | 0.1972343559 | 0.8817386452 |
| H3 | -2.3242662742 | 0.1956439791 | -0.8830393167 |
| C1 | -2.0602036256 | -0.3672349044 | -0.0003032812 |
| C2 | 0.1866163039 | 0.4720198900 | 0.0010030690 |
| C3 | 1.5697662153 | 0.0293497789 | 0.0000233394 |
| N | 2.6764708578 | -0.2925131631 | -0.0006957204 |
| O1 | -0.6762711321 | -0.6808119827 | -0.0009834169 |
| O2 | -0.1573444497 | 1.5969762157 | 0.0025455137 |

**C-O distance = 1.54 Å**

-320.71573013 -320.52992894 -320.50667197 -320.46397532 -320.45211552

| | | | |
|---|---|---|---|
| H1 | -2.5610173039 | -0.2629855700 | 0.8867306397 |
| H2 | -2.7017855921 | -1.7794084587 | -0.0059956656 |
| H3 | -2.5537489173 | -0.2520823907 | -0.8777497792 |
| C1 | 1.3495780703 | -0.0424298805 | -0.0006062479 |
| C2 | -0.0547908999 | 0.2953079074 | -0.0021670109 |
| C3 | -2.2494701481 | -0.8003333838 | 0.0023450822 |
| N | 2.4745991925 | -0.2929100829 | 0.0030241625 |
| O1 | -0.5194822818 | 1.3703236510 | -0.0105068118 |
| O2 | -0.8528771198 | -1.0217237917 | 0.0071006310 |

**C-O distance = 1.64 Å**

-320.69896695 -320.52300867 -320.51289384 -320.45585915 -320.43825796

| | | | |
|---|---|---|---|
| H1 | -2.6474332634 | -1.3098139559 | -0.0170497710 |
| H2 | -2.3327172907 | 0.1684318336 | 0.8926799796 |
| H3 | -2.3181722484 | 0.1973984614 | -0.8711766673 |
| C1 | -2.0792812023 | -0.3921102258 | 0.0032400494 |
| C2 | 0.2448430353 | 0.5418607535 | -0.0029773770 |
| C3 | 1.6025683852 | 0.0596801407 | 0.0001581959 |
| N | 2.6966744465 | -0.3008396607 | 0.0019400767 |
| O1 | -0.7236625329 | -0.7815642724 | 0.0089877873 |
| O2 | -0.1239993293 | 1.6527199256 | -0.0144422736 |

**C-O distance = 1.74 Å**

-320.68194676 -320.51777804 -320.51724787 -320.46937438 -320.44627888

| | | | |
|---|---|---|---|
| H1 | -2.5556954695 | -0.2441988221 | 0.8835705956 |

| | | | |
|---|---|---|---|
| H2 | -2.8010488153 | -1.7499323929 | 0.0011259590 |
| H3 | -2.5579096427 | -0.2436179507 | -0.8811387059 |
| C1 | 1.3873150482 | -0.0404836545 | -0.0025469445 |
| C2 | 0.0050426670 | 0.3545492491 | -0.0012169772 |
| C3 | -2.2778626376 | -0.8043739074 | 0.0006929448 |
| N | 2.4952446884 | -0.3575600773 | 0.0019938174 |
| O1 | -0.4563016931 | 1.4261623030 | 0.0008415174 |
| O2 | -0.9077791453 | -1.1267867473 | -0.0011472067 |

**C-O distance = 1.84 Å**

-320.66553306 -320.52086176 -320.51463933 -320.49396185 -320.43596816

| | | | |
|---|---|---|---|
| H1 | -2.7183523171 | -1.3094796407 | 0.0109047282 |
| H2 | -2.3276061342 | 0.1717719255 | 0.8808119340 |
| H3 | -2.3313768384 | 0.1574773153 | -0.8846541735 |
| C1 | -2.1035195055 | -0.4194447466 | 0.0023714811 |
| C2 | 0.3021845076 | 0.6153330246 | -0.0017482923 |
| C3 | 1.6421102853 | 0.1028976303 | -0.0027946265 |
| N | 2.7148486046 | -0.3195635107 | -0.0035943453 |
| O1 | -0.7752488527 | -0.8762147568 | 0.0030025023 |
| O2 | -0.0842197496 | 1.7129857591 | -0.0029392081 |

**C-O distance = 1.94 Å**

-320.65009365 -320.52423373 -320.52198428 -320.51597697 -320.42445756

| | | | |
|---|---|---|---|
| H1 | -2.5630543450 | -0.2640257330 | 0.8839577556 |
| H2 | -2.8750529821 | -1.7560144318 | 0.0015805893 |
| H3 | -2.5652421686 | -0.2646963722 | -0.8827759076 |
| C1 | 1.4280750609 | 0.0033476897 | -0.0024193766 |
| C2 | 0.0597136707 | 0.4267970838 | -0.0006218312 |
| C3 | -2.3064277506 | -0.8346606651 | 0.0005002601 |
| N | 2.5212566786 | -0.3637518991 | 0.0012176901 |
| O1 | -0.4085266130 | 1.4905169888 | 0.0017863316 |
| O2 | -0.9597365509 | -1.2237546610 | -0.0010505114 |

**C-O distance = 2.04 Å**

-320.63631087 -320.52828256 -320.52300199 -320.51394909 -320.41302095

| | | | |
|---|---|---|---|
| H1 | -2.7936119537 | -1.3113420487 | 0.0105969236 |

| | | | |
|---|---|---|---|
| H2 | -2.3403502617 | 0.1478946793 | 0.8858832516 |
| H3 | -2.3417920882 | 0.1376227822 | -0.8822795526 |
| C1 | -2.1380017903 | -0.4485436148 | 0.0050676627 |
| C2 | 0.3647637612 | 0.6811029080 | -0.0064062155 |
| C3 | 1.6940776548 | 0.1530262865 | -0.0039178545 |
| N | 2.7400298621 | -0.3325726827 | -0.0006146667 |
| O1 | -0.8381819421 | -0.9664239928 | 0.0070949930 |
| O2 | -0.0281132419 | 1.7749986831 | -0.0140645416 |

**C-O distance = 2.14 Å**

-320.62400900 -320.53904313 -320.52301142 -320.51457065 -320.40251265

| | | | |
|---|---|---|---|
| H1 | -2.5793032764 | -0.2867976697 | 0.8829093410 |
| H2 | -2.9522633462 | -1.7652762292 | 0.0021195194 |
| H3 | -2.5796575208 | -0.2917269746 | -0.8868772439 |
| C1 | 1.4827097004 | 0.0585854268 | -0.0005581744 |
| C2 | 0.1216641775 | 0.4946042289 | 0.0027368901 |
| C3 | -2.3439681398 | -0.8675194854 | -0.0004455844 |
| N | 2.5524079936 | -0.3716687975 | -0.0036994008 |
| O1 | -0.3494478546 | 1.5582628298 | 0.0054890474 |
| O2 | -1.0211367336 | -1.3147053291 | 0.0005006057 |

**C-O distance = 2.24 Å**

-320.61412653 -320.54763061 -320.52090032 -320.51296985 -320.38630275

| | | | |
|---|---|---|---|
| H1 | -2.5959867503 | -0.3107996795 | 0.8934496343 |
| H2 | -2.9933362183 | -1.7723373017 | -0.0058775779 |
| H3 | -2.5952396620 | -0.2958942367 | -0.8785525797 |
| C1 | 1.5195385545 | 0.0875823312 | -0.0000896342 |
| C2 | 0.1585161940 | 0.5258927073 | -0.0062194267 |
| C3 | -2.3708203538 | -0.8839287897 | 0.0026358716 |
| N | 2.5722705857 | -0.3794499134 | 0.0106590716 |
| O1 | -0.3054664709 | 1.5973665551 | -0.0127246250 |
| O2 | -1.0584708789 | -1.3546736726 | -0.0011057341 |

**C-O distance = 2.34 Å**

-320.60495077 -320.55387615 -320.51909446 -320.51264179 -320.38828707

| | | | |
|---|---|---|---|
| H1 | -2.6164672491 | -0.3074046563 | 0.8752382012 |

| | | | |
|---|---|---|---|
| H2 | -3.0369876810 | -1.7819401126 | 0.0101726602 |
| H3 | -2.6141193758 | -0.3336117138 | -0.8985175669 |
| C1 | 1.5554335256 | 0.1121910462 | 0.0020730807 |
| C2 | 0.1958978779 | 0.5570094030 | 0.0081921501 |
| C3 | -2.3999961868 | -0.9032881097 | -0.0027081125 |
| N | 2.6011577091 | -0.3708789276 | -0.0144623576 |
| O1 | -0.2567899402 | 1.6349775823 | 0.0154409782 |
| O2 | -1.0971236797 | -1.3932965115 | 0.0067459667 |

**C-O distance = 2.54 Å**

-320.59155602 -320.56169951 -320.51549457 -320.51183836 -320.39278218

| | | | |
|---|---|---|---|
| H1 | -2.6688687071 | -0.3662504417 | 0.8896461773 |
| H2 | -3.1133006601 | -1.8199945924 | 0.0008837671 |
| H3 | -2.6731591746 | -0.3645138793 | -0.8873419715 |
| C1 | 1.6307797196 | 0.1650069301 | -0.0033194877 |
| C2 | 0.2782947666 | 0.6335493999 | -0.0002137563 |
| C3 | -2.4644503138 | -0.9494852197 | 0.0000833365 |
| N | 2.6583475197 | -0.3572587207 | 0.0027847858 |
| O1 | -0.1460597679 | 1.7253852849 | 0.0030774080 |
| O2 | -1.1705783823 | -1.4526807611 | -0.0034252591 |

**C-O distance = 2.74 Å**

-320.58344578 -320.56579170 -320.51251904 -320.51096732 -320.39590979

| | | | |
|---|---|---|---|
| H1 | -2.7422467688 | -0.4149992635 | 0.8913802305 |
| H2 | -3.1879423871 | -1.8623682750 | -0.0071472711 |
| H3 | -2.7465741315 | -0.4026816126 | -0.8877552276 |
| C1 | 1.7105673028 | 0.2018406101 | 0.0029424839 |
| C2 | 0.3753417665 | 0.7191541120 | 0.0030519665 |
| C3 | -2.5385851085 | -0.9920005300 | -0.0027226951 |
| N | 2.7095442143 | -0.3742092968 | 0.0047936289 |
| O1 | -0.0036578334 | 1.8290546923 | 0.0070137496 |
| O2 | -1.2454420543 | -1.4900324365 | -0.0093818656 |

# TSSCDS calculations

The automated TSSCDS method has been presented elsewhere,[1, 2] and here only a brief summary is provided. It combines high-energy chemical dynamics (or trajectory) simulations (CDS) with the efficient Bond Breaking/Formation Search (BBFS) algorithm that searches for good guess transition states structures.

TSSCDS employs two levels of theory: a low level (LL) is used for the CDS step, as well as for an initial optimization of the TSs. Then, the structures are re-optimized at a high level (HL) of theory. As LL, one may typically employ a semiempirical method, and then, to refine the calculations, a HL (DFT or ab initio) is selected.

The BBFS algorithm that picks guess TS structures from the CDS snapshots plays a key role in the method. It selects the structure(s) where one or several bonds break or form along the trajectory, and it also determines which atoms are involved in the chemical process.[1, 2] More specifically, for each *jk* pair of atoms and step *i* along the trajectory, a normalized distance $\delta_{jk}^{\mathrm{i}}$ can be defined as $\delta_{jk}^{i} = d_{jk}^{i}/d_{jk}^{i,\mathrm{ref}}$, where $d_{jk}^{i}$ and $d_{jk}^{i,\mathrm{ref}}$ are the *jk* distance and some reference value, respectively. The algorithm considers that a reaction takes place when the following condition is fulfilled:[1, 2]

$$\max\left(\delta_{jn}^{\Delta t}\right) > \min\left(\delta_{jo}^{\Delta t}\right) \qquad (1)$$

Where the subscripts *n* and *o* run over the list of neighbors (atoms bonded to *j*) and outer atoms (non-bonded) of *j*, respectively. The superscript indicates that the inequality has to be held for at least a time window $\Delta t$, which is another parameter of the algorithm.

Once BFFS is performed, the procedure carries on optimizing the structure(s) selected by BFFS. The optimization is partial, with the atoms involved in the chemical reaction kept

frozen. The effect of this step is a relaxation of the normal modes perpendicular to the reaction coordinate, which leads to a structure of lower energy and, most likely, closer to the TS we are looking for.

Finally, the partially optimized structure is subjected to transition state optimization using the Eigenvector Following (EF) algorithm, which is implemented in the electronic structure programs interfaced with TSSCDS.

Table 2S collects the input parameters needed to carry out the TSSCDS calculations for this system. Two different batches of trajectories are run, with excitation energies of 300 and 450 kcal/mol, respectively. Like in previous work, a time window $\Delta t$ and simulation time $t^{CDS}$ of 20 and 500 fs, respectively, are selected.[1, 2]

**Table 2S:** Input parameters of the TSSCDS method employed in this work to find the stationary points of the $C_3H_3NO_2$ system.

<table>
<tr><td>$\Delta t$ (fs)[a]</td><td colspan="2">20</td></tr>
<tr><td>LL method</td><td colspan="2">PM7</td></tr>
<tr><td>HL method</td><td colspan="2">B3LYP/6-31+G(d,p) and MP2/6-311+G(2d,2p) optimizations and CCSD(T)/6-311+G(3df/2p) single point energy calculations (see text)</td></tr>
<tr><td>$E^{CDS}$ (kcal/mol)[b]</td><td colspan="2">300 and 450</td></tr>
<tr><td>$t^{CDS}$ (fs)[c]</td><td colspan="2">500</td></tr>
<tr><td rowspan="10">$d_{jk}^{i,ref,d}$</td><td>jk</td><td>$d_{jk}^{ref}$(Å)</td></tr>
<tr><td>CH</td><td>1.24</td></tr>
<tr><td>CC</td><td>1.63</td></tr>
<tr><td>CN</td><td>1.63</td></tr>
<tr><td>CO</td><td>1.63</td></tr>
<tr><td>NH</td><td>1.24</td></tr>
<tr><td>NO</td><td>1.63</td></tr>
<tr><td>OH</td><td>1.24</td></tr>
<tr><td>OO</td><td>1.63</td></tr>
<tr><td>HH</td><td>0.84</td></tr>
</table>

[a]Time window (for its definition see refs [1, 2]). [b]Energy of the chemical dynamics simulations. [c]Simulation time. [d]Reference distances (for the definition see refs [1, 2]).

For the trajectory calculations, as well as for a first optimization of TS structures the PM7 semiempirical Hamiltonian[3] is employed.

After the exploratory search at the LL, all stationary structures are re-optimized using the B3LYP/6-31+G(d,p) level of theory, and the energies refined with single point CCSD(T)/6-311+G(3df,2p) calculations. Vibrational frequencies are also calculated at the B3LYP/6-31+G(d,p) level of theory to confirm whether the structures correspond to minima or transition states.

Then, using the above DFT and *ab initio* data, a preliminary Kinetic Monte Carlo (KMC) simulation (*vide infra*) was carried out to identify the most important structures involved in the unimolecular fragmentation of the molecule at 148.12 kcal/mol, which corresponds to a photon wavelength of 193 nm.

The structures selected in the kinetic analysis (*vide infra*) are re-optimized at the MP2/6-311+G(2d,2p) level of theory, and, as above, their energies refined with single point CCSD(T)/6-311+G(3df,2p) calculations. Zero-point energy corrections and frequencies are calculated also at the MP2/6-311+G(2d,2p) level of theory for the selected structures (*vide infra*).

A total of 57 minima and 145 transition states are optimized in this study at the B3LYP/6-31+G(d,p) level of theory using TSSCDS. Transition states TS144 and TS145 were not found using the automated TSSCDS procedure. They correspond to torsional barriers, and were only optimized at the MP2/6-311+G(2d,2p) level of theory, after the TSSCDS procedure.

As indicated in previous work, TSSCDS is designed to search for bond breaking/formation,[1, 2] although some transition states for torsional rotations may be found due to deviation from the original target.

Figure 3S shows the typical stair-like increase[2] in the number of TSs as a function of the number of trajectories in the microcanonical ensembles.

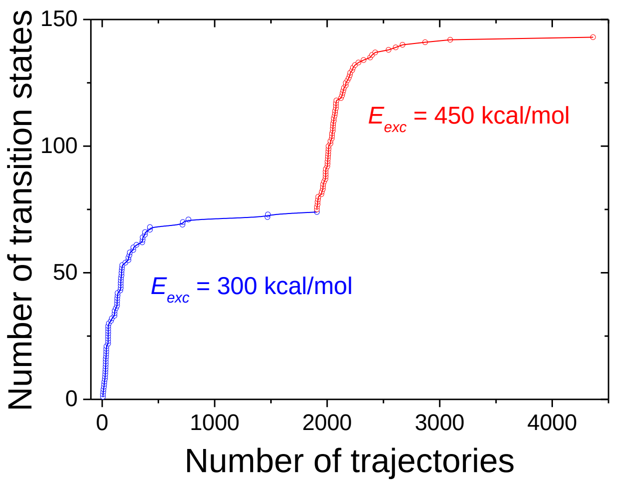


**Figure 3S.** Number of transition state structures found in this study as a function of the number of trajectories employed in just one iteration of the TSSCDS method.[2] Two different ensembles of trajectories are employed with excitation energies of 300 and 450 kcal/mol, respectively.

## List of minima

The following structures are optimized at the B3LYP/6-31+G(d,p) level of theory. ZPE is given in kcal/mol and is calculated at this level.

The geometry is in Å, and the energy (given in a.u.) is a CCSD(T)/6-311+G(3df,2p) single point calculation at the B3LYP/6-31+G(d,p) optimized geometry

```
MIN1
E= -320.8407519900 ZPE= 37.7148600000
O -0.886672 1.396590 -0.000028
C -2.113135 -0.682873 0.000200
H -2.105974 -1.333293 0.881117
H -2.106110 -1.333719 -0.880398
H -3.005818 -0.058041 0.000138
C -0.885477 0.186088 -0.000072
O 2.640866 -0.013855 0.000242
C 1.490364 -0.220871 -0.000041
N 0.319119 -0.575842 -0.000441
MIN2
E= -320.8356306600 ZPE= 38.1977100000
O 0.749610 1.275175 0.138155
```

C -0.291214 -0.881923 0.225423
H 1.599604 1.730776 0.008049
H -0.259246 -1.235202 1.264149
H -0.214815 -1.766583 -0.412759
C 0.966131 -0.044312 -0.000274
O 2.045221 -0.536305 -0.235852
C -1.565352 -0.202479 -0.008243
N -2.591656 0.304618 -0.197043
MIN3
E= -320.8199316400 ZPE= 39.6048500000
O -0.011787 -1.100088 0.000001
C 1.346065 -0.625386 0.000005
H 1.853544 -0.997672 -0.895459
H 1.853538 -0.997671 0.895472
H -0.243426 2.200662 -0.000003
C -0.834258 -0.008116 -0.000003
O -2.037339 -0.049697 -0.000006
C 0.096849 1.170237 -0.000001
N 1.325345 0.824651 0.000003
MIN4
E= -320.8082694300 ZPE= 37.9376900000
O -0.740468 -0.734678 0.000000
C -2.150976 -0.399866 0.000000
H -2.666584 -1.358146 0.000000
H -2.395836 0.178108 -0.893212
H -2.395836 0.178108 0.893212
C 0.099890 0.301583 0.000000
O -0.194748 1.473883 0.000000
C 1.493165 -0.167658 0.000000
N 2.612501 -0.473725 0.000000
MIN5
E= -320.8079552100 ZPE= 37.9282700000
O 0.741483 0.731134 0.000146
C 2.154783 0.401459 -0.000821
H 2.655175 1.333324 0.255597
H 2.451219 0.053514 -0.992641
H 2.361287 -0.370231 0.743260
C -0.100708 -0.304091 -0.001408
O 0.188621 -1.477805 0.001075
C -1.492635 0.169674 -0.000007
N -2.611022 0.479216 -0.000366
MIN6
E= -320.8077302800 ZPE= 37.9285300000
O 0.188024 -1.478522 -0.001880
C 2.153821 0.401412 0.005010
H 2.351938 -0.437343 -0.664065
H 2.470768 0.153999 1.020625
H 2.641779 1.308296 -0.347342
C -0.100577 -0.304617 0.000322
O 0.742192 0.730402 -0.006579
C -1.492183 0.169804 0.000614
N -2.610368 0.480058 0.003253
MIN7
E= -320.8045741600 ZPE= 37.2138900000
O 0.584026 1.393885 0.000001
C 2.104014 -0.514336 -0.000003

H 2.920502 0.206571 0.000064
H 2.166429 -1.157683 0.882710
H 2.166484 -1.157580 -0.882788
C 0.802348 0.222572 0.000000
O -0.268151 -0.737061 0.000006
C -1.492540 -0.283614 0.000001
N -2.609050 0.043766 -0.000004
MIN8
E= -320.8012158700 ZPE= 37.1877500000
O 1.969311 -0.700578 -0.000016
C 0.748119 1.400990 0.000004
H 0.179168 1.711274 -0.881928
H 0.179697 1.711270 0.882281
H 1.726820 1.879201 -0.000276
C 0.953542 -0.083133 -0.000012
O -0.260568 -0.877402 0.000026
C -1.424114 -0.300571 0.000003
N -2.488701 0.174055 -0.000019
MIN9
E= -320.8001941200 ZPE= 37.6665100000
O 1.151270 0.453078 -0.000150
C 1.668332 -0.899823 0.000079
H 1.348746 -1.435518 -0.896876
H 1.350652 -1.434344 0.898412
H 2.750532 -0.782105 -0.001148
C -0.165572 0.682968 -0.000005
O -0.638781 1.790724 0.000070
C -1.037186 -0.511844 -0.000004
N -1.763327 -1.418036 -0.000024
MIN10
E= -320.7963718800 ZPE= 37.9775800000
O -2.115300 -0.135448 0.000000
C 0.000000 0.958304 0.000000
H -0.248624 1.552509 0.884245
H -0.248624 1.552509 -0.884245
H 0.629119 -1.422254 0.000000
C -0.919514 -0.278483 0.000000
O -0.340186 -1.490171 0.000000
C 2.547468 0.433962 0.000000
N 1.392042 0.662784 0.000000
MIN11
E= -320.7939414400 ZPE= 37.3100600000
O -2.212630 -0.343937 0.000004
C -0.898391 -0.823265 0.000000
H -0.707182 -1.452673 -0.884092
H -0.707167 -1.452661 0.884099
H -2.181554 0.627719 -0.000039
C 0.113834 0.301901 -0.000003
O -0.210315 1.472949 0.000003
C 1.531293 -0.096644 0.000001
N 2.642719 -0.435205 -0.000002
MIN12
E= -320.7930242800 ZPE= 37.3790400000
O 0.342830 1.515435 -0.114618
C -0.065554 0.326725 0.496180
H 1.133045 1.306138 -0.646259

H 0.713914 -1.790787 0.707395
H -0.142760 0.471455 1.586819
C 0.948906 -0.808572 0.260843
O 1.950381 -0.603562 -0.384412
C -1.393025 -0.128742 0.022734
N -2.427407 -0.516894 -0.333465
MIN13
E= -320.7900924000 ZPE= 37.3007600000
O -1.517169 -1.147528 -0.223948
C -1.323360 0.192119 0.168913
H -1.189980 -1.753582 0.454130
H -1.956547 0.819674 -0.464075
H -1.611861 0.378841 1.215115
C 0.112109 0.688497 0.001513
O 0.413444 1.858057 -0.083308
C 1.159376 -0.361580 -0.006308
N 1.985634 -1.177626 0.038310
MIN14
E= -320.7880158900 ZPE= 37.0355800000
O -1.957033 -0.933976 0.145706
C -1.248439 -0.084454 -0.330201
H 1.069150 2.095209 0.255012
H -1.455253 0.415176 -1.296472
H -0.145243 0.404382 1.451006
C 0.036327 0.420586 0.367653
O 0.261918 1.726406 -0.129328
C 1.158680 -0.493408 0.069282
N 2.058979 -1.187221 -0.168710
MIN15
E= -320.7881028900 ZPE= 37.1298500000
O 2.196867 -0.198875 0.000000
C 0.910658 -0.757659 0.000001
H 0.710245 -1.383778 0.886297
H 2.851217 -0.908818 -0.000003
H 0.710244 -1.383777 -0.886295
C -0.122187 0.353096 0.000002
O 0.109071 1.537709 -0.000002
C -1.522335 -0.143990 0.000008
N -2.616575 -0.534711 -0.000006
MIN16
E= -320.7849281600 ZPE= 36.9475700000
O -2.188175 0.152097 0.000000
C 2.492795 0.373724 0.000000
H 0.355745 -1.496354 0.000000
H 3.035871 0.297923 0.935997
H 3.035871 0.297923 -0.935997
C -1.027074 -0.142420 0.000000
O -0.613897 -1.429473 0.000000
C 1.199128 0.600531 0.000000
N 0.000000 0.875501 0.000000
MIN17
E= -320.7831508100 ZPE= 37.6874200000
O 0.123033 1.464093 -0.000007
C 2.109066 -0.367398 0.000011
H 2.342360 0.215642 -0.893000
H 2.645736 -1.314263 -0.000543

H 2.342563 0.214641 0.893630
C -0.145994 0.289325 0.000002
O 0.707934 -0.733400 -0.000029
C -2.592809 -0.519127 0.000002
N -1.457139 -0.196909 0.000016
MIN18
E= -320.7805677800 ZPE= 37.4114900000
O -0.099173 -1.471730 0.002039
C -2.143871 0.368310 -0.004717
H -2.677611 1.093929 0.607652
H -2.224985 -0.643852 0.393249
H -2.502126 0.403134 -1.036298
C 0.152641 -0.293565 0.000920
O -0.703536 0.727467 0.010354
C 2.592559 0.536585 -0.004817
N 1.459775 0.204702 -0.001724
MIN19
E= -320.7813308500 ZPE= 38.3094700000
O -1.587872 -0.879950 -0.218251
C -2.028986 0.493626 -0.125530
H -2.907687 0.657496 0.495398
H -0.708335 -0.120445 1.557793
H -1.980517 1.051006 -1.058591
C -0.773093 0.048105 0.483800
O 2.775545 -0.138765 -0.039834
C 1.618597 0.076284 -0.033243
N 0.456578 0.407653 -0.125725
MIN20
E= -320.7761588100 ZPE= 37.4962100000
O 1.003391 0.644272 0.000049
C 1.801760 -0.562246 -0.000005
H 1.605439 -1.153516 -0.896991
H 1.605259 -1.153721 0.896808
H 2.831620 -0.209121 0.000138
C -0.328853 0.597697 -0.000023
O -1.028496 1.572277 0.000027
C -1.434067 -1.745225 0.000130
N -0.867789 -0.708200 -0.000168
MIN21
E= -320.7725894800 ZPE= 37.7286100000
O 0.508437 0.560677 -0.437815
C -0.733549 0.895656 0.167020
H -1.088117 1.790944 -0.345123
H -0.609293 1.104743 1.235610
H 1.016338 -0.393032 1.327894
C 1.381719 -0.179334 0.307352
O 2.438554 -0.536173 -0.126116
C -2.494550 -0.995821 -0.107902
N -1.688082 -0.145956 0.013463
MIN22
E= -320.7689984000 ZPE= 37.1354800000
O -1.698479 -0.858162 -0.223965
C -1.224601 0.404084 0.176899
H -1.397822 -1.541535 0.390075
H -1.726963 1.154813 -0.437433
H -1.453492 0.630659 1.230433

C 0.276964 0.625044 0.001984
O 0.795183 1.707818 -0.094038
C 1.690650 -1.551394 0.033237
N 1.049509 -0.558226 0.012605
MIN23
E= -320.7636877100 ZPE= 37.0579600000
O 1.976038 -0.610049 0.003816
C 0.765251 1.444610 -0.001734
H 1.799086 -1.500003 0.343678
H 1.672952 2.025613 0.087194
H -0.186573 1.949487 -0.095873
C 0.850209 0.120299 -0.007751
O -0.261903 -0.762261 -0.084211
C -1.461170 -0.272130 -0.005538
N -2.560612 0.106673 0.056900
MIN24
E= -320.7632569800 ZPE= 37.4752600000
O -0.982967 -0.621490 0.841428
C -1.102666 -0.884981 -0.585938
H -2.048168 -0.579228 -1.030826
H -0.699277 -1.841573 -0.910733
H -1.429489 1.645741 0.131013
C -0.217466 0.166052 -0.047437
O -0.501590 1.515478 -0.115328
C 1.229658 -0.047583 -0.018122
N 2.370891 -0.253968 -0.012753
MIN25
E= -320.7616392600 ZPE= 37.3990700000
O -0.529925 1.514314 0.002633
C -1.174701 -0.813079 -0.606598
H 0.051595 1.998797 -0.601152
H -0.832355 -1.780137 -0.968954
H -2.093828 -0.413289 -1.028580
C -0.225632 0.160669 -0.025618
O -1.028149 -0.605816 0.821639
C 1.211116 -0.132453 -0.000858
N 2.353498 -0.337740 -0.028149
MIN26
E= -320.7587775900 ZPE= 37.8500500000
O -1.437620 -1.152900 0.000001
C 1.887899 -0.572939 0.000004
H 2.316548 -0.954560 0.924063
H -0.739855 -1.827428 -0.000028
H 2.316543 -0.954586 -0.924046
C -0.900436 0.087850 -0.000002
O -1.573104 1.084517 0.000003
C 0.594445 0.102366 0.000004
N 1.528731 0.939997 -0.000008
MIN27
E= -320.7553463400 ZPE= 37.2166200000
O -1.528080 1.182579 -0.178212
C 2.592214 -0.030764 -0.294801
H 3.103889 0.912088 -0.455945
H 3.075097 -0.976388 -0.516380
H -2.477922 -0.914190 -0.484784
C -0.998747 0.115712 0.062261

O -1.587682 -1.088256 -0.133103
C 0.309535 -0.017195 0.701573
N 1.401002 -0.026087 0.161918
MIN28
E= -320.7576827500 ZPE= 39.3711100000
O 0.070166 -1.081963 0.000002
C -1.282581 -0.724401 0.000005
H -2.082966 1.304793 0.000004
H -1.784569 -1.094341 0.900506
H -1.784574 -1.094344 -0.900491
C 0.862812 0.082931 -0.000003
O 2.057582 0.018347 -0.000006
C -0.044793 1.318991 -0.000003
N -1.226072 0.761100 0.000002
MIN29
E= -320.7506090400 ZPE= 37.0795800000
O -0.234231 1.535529 -0.107199
C -2.184851 -0.547068 -0.021225
H -2.889010 -1.374850 -0.002160
H -0.448157 1.907451 0.762534
H -2.579884 0.469009 -0.103659
C 1.306614 -0.206909 0.006080
O 2.434295 -0.509410 -0.010899
C 0.017734 0.171290 0.018702
N -0.931492 -0.816349 0.038104
MIN30
E= -320.7500884500 ZPE= 37.0566500000
O -1.789051 -0.929703 -0.251582
C 2.562261 0.007548 -0.285778
H 3.038900 -0.843417 -0.760558
H 3.079998 0.956044 -0.187263
H -1.383329 -1.749365 0.073346
C -1.006361 0.137387 0.048879
O -1.381195 1.271881 -0.122932
C 0.279051 -0.208004 0.692878
N 1.373814 -0.103183 0.162101
MIN31
E= -320.7437312000 ZPE= 37.1274400000
O 2.814240 -0.237809 0.000001
C -2.067967 -0.826979 0.000000
H -1.668487 -1.306009 0.895119
H -1.668507 -1.306002 -0.895131
H -3.156428 -0.842395 0.000012
C -0.483229 1.038482 0.000000
O -1.708784 0.593029 0.000001
C 1.655334 -0.071210 0.000000
N 0.432134 -0.032730 -0.000001
MIN32
E= -320.7274724600 ZPE= 36.4183200000
O -1.007301 1.326417 -0.000079
C 2.201289 0.459111 0.000055
H 2.642468 0.778546 0.941157
H 2.642367 0.778866 -0.940987
H -2.686059 0.155641 0.000252
C -1.594189 0.280990 0.000074
O -1.027670 -0.976201 0.000027

C 0.333760 -1.201627 -0.000123
N 1.147976 -0.249375 -0.000006
MIN33
E= -320.7240464500 ZPE= 36.6608400000
O -1.271557 1.235985 -0.108432
C -1.748576 -0.070154 0.027153
H -2.310490 -0.220886 0.959519
H -2.422086 -0.247603 -0.815324
H -0.763734 1.498781 0.671936
C 1.401779 0.055981 0.005377
O 2.526111 0.399436 -0.005867
C 0.476698 -0.988199 -0.008503
N -0.759933 -1.157061 -0.006557
MIN34
E= -320.7143857700 ZPE= 36.3896700000
O 0.506809 1.391657 -0.000037
C 2.083732 -0.475580 0.000086
H 2.876000 0.272064 -0.001498
H 2.169031 -1.115960 -0.882603
H 2.170079 -1.113089 0.884774
C 0.759498 0.227052 -0.000079
O -0.263121 -0.774405 -0.000164
C -2.621741 0.080335 0.000133
N -1.499077 -0.281695 0.000014
MIN35
E= -320.7123693200 ZPE= 37.2988500000
O 1.571485 1.044781 0.000139
C -1.824070 -0.522346 0.000203
H -2.150299 -0.983253 0.929751
H 0.537002 -1.804837 -0.000442
H -2.150251 -0.983881 -0.929052
C 0.855864 0.086741 0.000021
O 1.284764 -1.185429 -0.000101
C -1.547091 1.039100 -0.000358
N -0.570666 0.182312 0.000034
MIN36
E= -320.7113908300 ZPE= 36.8661600000
O 1.389704 -0.393983 0.000027
C 2.674798 0.282301 0.000002
H 3.204279 -0.043697 -0.895614
H 3.204441 -0.044019 0.895404
H 2.520037 1.361712 0.000214
C 0.347506 0.370877 -0.000031
O -0.710375 -0.547053 -0.000021
C -1.907704 -0.024315 -0.000001
N -3.007283 0.354446 0.000019
MIN37
E= -320.7104713000 ZPE= 36.4515300000
O -1.939644 -0.695835 -0.000085
C -0.715848 1.405402 0.000031
H -1.698214 1.875959 -0.000116
H -0.149321 1.718542 -0.881799
H -0.149590 1.718529 0.882037
C -0.919874 -0.078564 -0.000001
O 0.267902 -0.893562 0.000113
C 2.531416 0.184004 -0.000091

N 1.428129 -0.237558 0.000003
MIN38
E= -320.7096388200 ZPE= 36.7992700000
O 0.901852 -0.245018 0.000005
C 2.332452 -0.501206 -0.000002
H 2.549362 -1.083199 0.895812
H 2.869895 0.447475 -0.000099
H 2.549322 -1.083354 -0.895724
C 0.533838 0.997998 -0.000001
O -0.854217 1.021387 0.000001
C -1.580537 -0.080361 -0.000001
N -2.294882 -0.998636 -0.000001
MIN39
E= -320.7090343100 ZPE= 37.1311800000
O -2.131006 0.758154 -0.170673
C -1.726515 -0.516327 0.100276
H -1.571438 1.367580 0.345697
H -1.865743 -0.829917 1.141117
H -2.191523 -1.206656 -0.601126
C 0.453450 0.332179 0.218095
O -0.248456 -0.697253 -0.126372
C 1.857371 0.092424 0.013214
N 3.022652 0.104590 -0.071262
MIN40
E= -320.7073493000 ZPE= 36.6804200000
O -1.562556 0.660830 0.000000
C -2.105183 -0.709366 0.000000
H -1.770938 -1.230810 -0.896586
H -3.183673 -0.571317 0.000072
H -1.770822 -1.230862 0.896512
C -0.316605 0.972503 -0.000001
O 0.414323 -0.253075 0.000001
C 1.715411 -0.145102 0.000000
N 2.878508 -0.133895 -0.000001
MIN41
E= -320.7069920600 ZPE= 37.1665600000
O -2.410505 -0.574280 -0.280177
C -1.634740 0.485969 0.123837
H -1.579797 1.217306 -0.682140
H -1.945795 0.923809 1.077303
H -2.614973 -1.151955 0.468307
C 0.662217 0.509888 -0.403798
O -0.253039 0.021238 0.379617
C 1.954176 -0.035569 -0.053858
N 3.079856 -0.332364 0.049132
MIN42
E= -320.7040049800 ZPE= 37.8020400000
O -2.106211 -0.638656 -0.045667
C 1.742465 -0.234208 -0.614803
H -2.842094 -0.003394 0.025182
H 2.393692 0.580532 -0.925451
H 1.951960 -1.211675 -1.044926
C 0.444937 0.074192 -0.055045
O 1.453260 -0.253300 0.841130
C -0.962592 0.027794 -0.054584
N -0.518402 1.223359 -0.010273

MIN43
E= -320.7019159400 ZPE= 37.0673300000
O -1.139048 -1.204498 -0.403105
C -1.376671 -0.143819 0.424659
H -2.433478 0.110366 0.394515
H -0.290135 -1.624524 -0.197300
H -1.000370 -0.269532 1.444573
C 0.544873 1.261923 -0.267964
O -0.722337 1.140125 -0.071014
C 1.351718 0.079511 0.006323
N 2.213649 -0.698145 0.167580
MIN44
E= -320.7001383300 ZPE= 36.3664400000
O -0.322222 1.460399 -0.000008
C -2.151490 -0.499776 -0.000012
H 0.437900 2.058264 0.000029
H -2.751458 -1.394468 -0.000008
H -2.515621 0.515827 -0.000018
C 0.096010 0.162431 0.000023
O -0.854771 -0.729628 0.000011
C 1.429300 -0.241114 -0.000002
N 2.571743 -0.507863 -0.000010
MIN45
E= -320.6999687400 ZPE= 36.8571500000
O 2.399104 -0.396907 -0.092880
C 1.040606 -0.499209 0.000810
H 2.775869 -0.073372 0.737580
H 0.662340 -1.007875 -0.885616
H 0.675654 -0.955701 0.926360
C -0.817368 1.126383 -0.009684
O 0.452116 0.893082 -0.013284
C -1.681788 -0.043816 0.002535
N -2.596046 -0.776085 0.015575
MIN46
E= -320.6920660200 ZPE= 36.2114300000
O -1.483224 -0.139672 0.239976
C -1.152581 1.242172 -0.172253
H -2.124537 1.724213 -0.250283
H -0.643700 1.229952 -1.135080
H -0.538593 1.711429 0.593570
C -0.824086 -1.235419 0.154354
O 0.542896 -1.077923 -0.277429
C 1.332797 -0.068548 -0.035999
N 2.098953 0.777990 0.202115
MIN47
E= -320.6913883500 ZPE= 37.0189900000
O -2.144704 -0.708890 -0.227520
C -1.641584 0.513970 0.136436
H -1.745622 -1.388930 0.338432
H -2.116776 1.284903 -0.466399
H -1.713697 0.723912 1.207877
C 0.528885 -0.281880 0.370563
O -0.195434 0.640375 -0.194627
C 3.016689 -0.138134 -0.141110
N 1.839038 -0.090785 0.014563
MIN48

E= -320.6851283800 ZPE= 36.7967700000
O 1.376803 1.070173 0.410985
C 1.293270 0.031452 -0.480791
H 0.570147 1.604583 0.383018
H 2.287765 -0.377567 -0.641335
H 0.788919 0.283572 -1.417844
C -0.730378 -1.159402 0.305327
O 0.544569 -1.148249 0.083468
C -2.170082 0.904211 -0.181136
N -1.339238 0.065207 -0.019980
MIN49
E= -320.6829304400 ZPE= 36.7702600000
O 1.609243 0.934943 -0.399296
C 1.193635 0.056864 0.577292
H 2.318995 0.538709 -0.924240
H 0.524758 0.588746 1.251917
H 2.008359 -0.442310 1.106596
C -0.811337 -1.076013 -0.342630
O 0.452640 -1.090540 -0.022654
C -2.262754 0.970965 0.110925
N -1.437778 0.121248 -0.018884
MIN50
E= -320.6819075600 ZPE= 36.7105800000
O -0.618417 1.140546 -0.000005
C 0.904340 1.190681 0.000016
H 1.227662 1.696672 0.910112
H 1.227694 1.696741 -0.910031
H -2.519114 -0.256327 0.000103
C -0.626495 -0.165761 -0.000051
O -1.733455 -0.838490 0.000012
C 0.906394 -0.387411 -0.000021
N 1.681900 -1.339798 0.000014
MIN51
E= -320.6776219700 ZPE= 36.6497900000
O 1.139641 -0.432985 -0.000001
C 2.574589 -0.318530 0.000001
H 2.938337 -1.346765 -0.000004
H 2.913974 0.206025 -0.897117
H 2.913973 0.206015 0.897125
C -1.735064 -0.049139 -0.000002
O -2.813921 -0.504347 -0.000006
C -0.717892 0.806067 0.000004
N 0.556880 0.829000 0.000005
MIN52
E= -320.6718798800 ZPE= 36.2959000000
O 1.947910 -0.598288 0.002716
C 0.720015 1.449333 -0.003259
H 1.623955 2.033507 0.101543
H 1.798225 -1.453102 0.435370
H -0.232106 1.947854 -0.113554
C 0.816133 0.126374 -0.010318
O -0.268832 -0.786513 -0.102460
C -2.592806 0.120658 0.074489
N -1.468964 -0.232576 0.001303
MIN53
E= -320.6590394200 ZPE= 35.8848900000

O 2.223205 0.630180 -0.015387
C -2.792665 0.048364 -0.033371
H -3.360994 -0.093587 0.882781
H -3.308194 0.110973 -0.988719
H 3.191491 0.620963 -0.028381
C 1.837130 -0.635604 -0.018082
O 0.505348 -0.722273 -0.001057
C -0.320278 0.432393 0.080422
N -1.527978 0.146782 0.013150
MIN54
E= -320.6359135600 ZPE= 35.0002600000
O 1.099424 -0.592662 -0.000055
C 2.474319 -0.359607 0.000034
H 2.816071 0.167720 0.902430
H 2.816153 0.167906 -0.902222
H 2.936661 -1.360433 -0.000052
C -0.875272 0.995538 0.000007
O 0.324024 1.016245 -0.000011
C -1.780200 -0.084177 0.000006
N -2.695650 -0.810625 0.000013
MIN55
E= -320.6233550100 ZPE= 35.6472800000
O 0.892166 -0.259502 -0.000078
C 2.328342 -0.476674 0.000029
H 2.562211 -1.053577 0.895105
H 2.843516 0.484250 0.001056
H 2.562667 -1.051941 -0.895982
C 0.488789 0.971070 0.000038
O -0.855506 1.026026 0.000010
C -2.351915 -1.056004 0.000067
N -1.578994 -0.163041 -0.000064
MIN56
E= -320.6157662300 ZPE= 35.0816200000
O -1.591981 -0.581528 -0.000066
C -2.573777 0.436901 0.000116
H -3.516305 -0.123182 0.000114
H -2.521943 1.055255 -0.903099
H -2.521821 1.055056 0.903460
C 0.733869 -0.629497 0.000143
O -0.207468 0.185101 -0.000237
C 2.011263 0.003143 0.000021
N 3.132506 0.331572 0.000040
MIN57
E= -320.5761436000 ZPE= 34.4279100000
O 2.494574 -0.595079 0.164850
C 1.523839 0.758521 -0.250487
H 1.591696 1.262844 0.725121
H 2.876238 -0.874912 -0.681012
H 1.980595 -1.339200 0.533337
C -0.766020 0.715813 0.270123
O 0.262127 0.081165 -0.237973
C -1.964166 -0.042511 0.023933
N -3.037722 -0.504050 -0.036269

The following structures are re-optimized at the MP2/6-311+G(2d,2p) level of theory. ZPE is given in kcal/mol and is calculated at this level. They are selected after a preliminary KMC calculation, and are employed in the second KMC simulation.

The geometry is in Å, the energy (given in a.u.) is a CCSD(T)/6-311+G(3df,2p) single point calculation at the MP2/6-311+G(2d,2p) optimized geometry

The frequencies are given in $cm^{-1}$.

```
MIN4
E= -320.80818873  ZPE= 38.05827
O        0.474684   -0.936721    0.000000
C        1.921193   -1.007573    0.000000
H        2.148910   -2.063589    0.000000
H        2.313330   -0.522866    0.886512
H        2.313330   -0.522866   -0.886512
C        0.000000    0.309654    0.000000
O        0.648198    1.329007    0.000000
C       -1.468994    0.291514    0.000000
N       -2.638830    0.344210    0.000000
Freqs: 142,  167,  168,  311,  329,  537,  589,  766,  866,
1011, 1192, 1220, 1285, 1495, 1517, 1524, 1761, 2168, 3115,
3211, 3247
MIN9
E= -320.80016544  ZPE= 37.79401
O        1.168523    0.432094   -0.000007
C        1.595179   -0.950230    0.000002
H        1.242858   -1.458634   -0.890983
H        1.242346   -1.458805    0.890685
H        2.674917   -0.905250    0.000321
C       -0.141812    0.698667    0.000002
O       -0.586483    1.817126    0.000001
C       -1.030240   -0.482217    0.000005
N       -1.765029   -1.395485   -0.000004
Freqs: 118,  158,  166,  270,  338,  524,  629,  747,  748,
1061, 1181, 1189, 1279, 1508, 1523, 1531, 1774, 2148, 3106,
3202, 3237
MIN17
E= -320.78332436  ZPE= 37.86995
O         0.150306    1.456902    0.000000
C         2.093050   -0.369139    0.000001
H         2.316407    0.211590   -0.887132
H         2.634583   -1.303815    0.000021
H         2.316397    0.211622    0.887115
C        -0.131322    0.290346    0.000000
O         0.695025   -0.749056   -0.000001
C        -2.597780   -0.504151    0.000001
N        -1.459104   -0.183500    0.000000
```

Freqs: 118, 138, 160, 225, 303, 537, 600, 772, 882, 1026, 1195, 1221, 1270, 1498, 1518, 1525, 1812, 2111, 3117, 3214, 3248

MIN20

E= -320.77642176 ZPE= 37.68704

| | | | |
|---|---|---|---|
| O | 0.948022 | -0.729125 | -0.000039 |
| C | 1.790870 | 0.446554 | -0.000015 |
| H | 1.614664 | 1.039245 | 0.890127 |
| H | 1.614639 | 1.039300 | -0.890116 |
| H | 2.798737 | 0.056858 | -0.000041 |
| C | -0.374645 | -0.594162 | -0.000012 |
| O | -1.149592 | -1.503174 | -0.000028 |
| C | -1.209751 | 1.877263 | 0.000076 |
| N | -0.807760 | 0.763580 | 0.000039 |

Freqs: 124, 133, 157, 189, 334, 542, 627, 754, 758, 1052, 1182, 1191, 1265, 1509, 1525, 1530, 1836, 2088, 3113, 3212, 3241

## List of transition states

The different channels obtained in this study (identified with IRC calculations at the B3LYP/6-31+G(d,p) level of theory, and also MP2/6-311+G(2d,2p) for the selected TSs; see below) can be grouped in the following 13 categories (below min*x* and min*y* refer to any of the 57 different minima):

(1) **Bim(trim) channel:** A+B (+C)↔D+E(+F), where two (or three) reactants are connected with two (or three) products.

(2) **$CH_2$ channel:** min*x*→$CH_2$ + $C_2HNO_2$.

(3) **$CH_2O$ channel:** min*x*→$CH_2O$ + $C_2HNO$.

(4) **CN channel:** min*x*→CN + $C_2H_3O_2$.

(5) **CO channel**: min*x*→CO + $C_2H_3NO$.

(6) **$CO_2$ channel**: min*x*→$CO_2$ + $C_2H_3N$.

(7) **$H_2$ channel**: min*x*→$H_2$ + $C_3HNO_2$.

(8) **HCN(HNC) channel:** min*x*→HCN(HNC) + $C_2H_2O_2$.

(9) **HNCO channel:** min*x*→HNCO + $C_2H_2O$.

(10) **HOCN channel:** min*x*→HOCN + $C_2H_2O$.

(11) **Iso channel:** min*x*↔min*y*. Isomerization reaction between minima *x* and *y*.

(12) **Triple 1:** min*x*→HCN(HNC) + $CH_2O$ + CO.

(13) **Triple 2:** min*x*→$H_2$ + HCO + NCCO.

A total of 41, 3, 10, 1, 9, 6, 11, 2, 1, 4, 49, 5, and 1 transition states are found for channels 1-13, respectively.

The following structures are optimized at the B3LYP/6-31+G(d,p) level of theory. The information of each transition state includes: the electronic energy (in a.u.), the zero-point energy (ZPE, in kcal/mol), the mechanism, and the Cartesian coordinates (in Å).

The energy is a CCSD(T)/6-311+G(3df,2p) single point calculation at the B3LYP/6-31+G(d,p) optimized geometry.

```
TS 1
 MIN 4 <--> MIN 4
E= -320.8064110900 ZPE= 37.7954300000
O 0.747890 -0.710930 0.000002
C 2.167926 -0.411654 -0.000001
H 2.589155 -0.871156 -0.895191
H 2.589159 -0.871161 0.895185
H 2.330444 0.665466 0.000001
C -0.104595 0.316908 0.000001
O 0.158994 1.496320 0.000000
C -1.488674 -0.179985 0.000000
N -2.601681 -0.508270 -0.000001
TS 2
 MIN 17 <--> MIN 17
E= -320.7812762900 ZPE= 37.5319900000
O 0.716505 -0.709210 0.000000
C 2.127339 -0.376134 0.000000
H 2.263693 0.704676 0.000000
H 2.560647 -0.824782 -0.895060
H 2.560648 -0.824783 0.895059
C -0.151219 0.302732 0.000000
O 0.084926 1.484415 0.000000
C -2.581282 -0.556033 0.000000
N -1.452210 -0.211448 0.000000
TS 3
 CO+C2H3NO <--> CO+C2H3NO
E= -320.7761436800 ZPE= 34.8830100000
O -0.835095 -0.406085 -0.095264
C -1.754813 -1.534109 0.023189
H -2.491489 -1.490930 -0.781770
H -2.241784 -1.507509 1.000255
H -1.128197 -2.418756 -0.072774
C 3.098832 0.131953 -0.633655
O 3.177418 -0.054692 0.485507
C -1.373556 0.766883 -0.008555
N -1.814270 1.845008 0.063781
TS 4
 MIN 19 <--> MIN 19
E= -320.7797255100 ZPE= 38.2401800000
O -1.855032 -0.373572 -0.549184
C -1.579332 0.871158 0.126378
H -2.367603 1.228245 0.787316
H -1.097322 -0.938773 1.341565
H -1.086684 1.624575 -0.485581
C -0.851463 -0.366830 0.448796
O 2.663016 0.335167 -0.082569
C 1.559174 -0.071331 -0.011212
N 0.473923 -0.600684 0.003850
TS 5
 HOCN+C2H2O <--> HOCN+C2H2O
```

E= -320.7621083200 ZPE= 34.1728300000
O -1.060988 -0.542403 0.000028
C -3.306421 0.524602 -0.000016
H -3.387331 1.604851 -0.000086
H 0.771629 -0.944452 -0.000010
H -4.193698 -0.096622 0.000044
C -2.122441 -0.035086 0.000006
O 1.745809 -1.025294 -0.000024
C 2.304609 0.145854 -0.000003
N 2.868050 1.166512 0.000014
TS 6
MIN 21 <--> MIN 21
E= -320.7673324900 ZPE= 37.5504800000
O 0.608397 0.819048 0.000000
C -0.806820 1.006359 0.000000
H 0.505547 -1.251158 -0.000002
H -1.055511 1.582583 0.894907
H -1.055510 1.582583 -0.894909
C 1.205902 -0.406324 0.000000
O 2.401937 -0.505759 0.000000
C -2.301882 -1.118480 0.000000
N -1.580056 -0.187092 0.000000
TS 7
MIN 24 <--> MIN 25
E= -320.7608609500 ZPE= 37.2053300000
O -0.963184 -0.684926 0.823874
C -1.140127 -0.830052 -0.598025
H -0.748849 -1.749136 -1.029508
H -0.877974 1.824722 -0.798509
H -2.099820 -0.480859 -0.977256
C -0.221468 0.171161 -0.017629
O -0.538060 1.515867 0.051823
C 1.222959 -0.072376 -0.019159
N 2.366917 -0.264951 -0.055917
TS 8
MIN 16 <--> CO2+C2H3N
E= -320.7488933200 ZPE= 33.9742000000
O -2.159618 -0.215873 0.000000
C 2.096793 0.302691 0.000000
H 0.807364 1.027170 0.000000
H 2.643164 0.494367 -0.921800
H 2.643164 0.494367 0.921800
C -1.032184 0.153421 0.000000
O -0.389845 1.234517 0.000000
C 1.199254 -0.737938 0.000000
N 0.102690 -1.210586 0.000000
TS 9
MIN 8 <--> HNCO+C2H2O
E= -320.7439124900 ZPE= 33.4766100000
O 2.094481 -0.683495 -0.001410
C 0.610764 1.367980 0.001238
H -0.606125 1.165353 -0.000887
H 0.832444 1.933087 0.911801
H 0.835530 1.936822 -0.906232
C 1.336761 0.175744 -0.000041
O -0.741848 -1.354501 0.001536

C -1.518769 -0.423041 -0.000130
N -2.065064 0.649229 -0.001728
TS 10
MIN 31 <--> MIN 31
E= -320.7418800000 ZPE= 36.9621900000
O -2.836792 0.237375 0.000004
C 2.136796 0.800500 0.000001
H 2.746898 0.929802 0.894587
H 1.285513 1.479538 0.000034
H 2.746842 0.929822 -0.894621
C 0.462087 -1.021291 -0.000001
O 1.693535 -0.595568 0.000003
C -1.675939 0.081779 -0.000001
N -0.452980 0.051494 -0.000007
TS 11
MIN 7 <--> HOCN+C2H2O
E= -320.7265988300 ZPE= 33.7405800000
O 2.089415 -1.248211 -0.000011
C 1.491795 1.225444 -0.000026
H 1.879114 1.694587 -0.909905
H 1.879024 1.694577 0.909898
H 0.320014 1.174511 -0.000073
C 1.788221 -0.150512 -0.000015
O -0.764132 0.098748 0.000093
C -2.013032 -0.059233 0.000029
N -3.183189 -0.208882 -0.000072
TS 12
MIN 4 <--> MIN 17
E= -320.7285793000 ZPE= 36.2118000000
O 0.083542 1.458141 -0.018179
C -2.052681 -0.262495 -0.011917
H -2.231164 0.328083 -0.912193
H -2.629013 -1.185106 -0.024987
H -2.274706 0.327914 0.878749
C 0.223829 0.277391 0.030090
O -0.662726 -0.695506 0.021252
C 1.744756 -0.406144 0.637151
N 1.753276 -0.460641 -0.556871
TS 13
MIN 9 <--> MIN 20
E= -320.7257637800 ZPE= 36.2712700000
O -0.743019 -0.831998 -0.017521
C -1.876505 0.075959 0.006183
H -1.857756 0.714023 -0.876908
H -1.853386 0.673486 0.918190
H -2.741002 -0.585327 -0.004172
C 0.505175 -0.447919 0.017869
O 1.485610 -1.106108 -0.004812
C 0.676676 1.287966 0.642179
N 0.668478 1.315234 -0.550833
TS 14
MIN 13 <--> MIN 22
E= -320.7218279200 ZPE= 35.8390700000
O -1.859996 -0.312313 -0.174446
C -1.009054 0.744764 0.130356
H -1.631445 -1.081386 0.367949

H -1.258756 1.580853 -0.529843
H -1.101328 1.092140 1.173433
C 0.483100 0.495780 -0.034206
O 1.381794 1.248619 -0.065876
C 0.849032 -1.287974 -0.616145
N 0.839811 -1.256783 0.575858
TS 15
MIN 4 <--> MIN 4
E= -320.7200315700 ZPE= 35.8930900000
O -0.489023 -1.100738 -0.015538
C -2.321025 -0.000017 0.018128
H -2.391789 -0.000321 1.097662
H -2.582061 0.918919 -0.487410
H -2.582030 -0.918682 -0.487922
C 0.112311 0.000013 -0.012633
O -0.489000 1.100773 -0.015537
C 1.577470 -0.000007 0.001303
N 2.738218 -0.000019 0.012213
TS 16
MIN 33 <--> CH2O+C2HNO
E= -320.7015056900 ZPE= 32.9637100000
O -1.025235 1.254123 -0.000022
C -1.790339 0.207487 0.000023
H -2.332913 -0.019963 0.923752
H -2.332999 -0.019972 -0.923652
H 0.162653 0.941597 0.000010
C 1.239442 0.140351 0.000003
O 2.400386 0.349636 0.000005
C 0.393059 -1.128854 -0.000003
N -0.792988 -1.292234 -0.000016
TS 17
MIN 40 <--> MIN 40
E= -320.7049116200 ZPE= 36.4882100000
O -1.548506 0.655498 -0.000001
C -2.171624 -0.681300 -0.000001
H -1.425573 -1.470744 -0.000018
H -2.791000 -0.715414 -0.895469
H -2.790976 -0.715429 0.895483
C -0.300019 0.952371 0.000000
O 0.437709 -0.270472 0.000003
C 1.737101 -0.150390 0.000000
N 2.900168 -0.128958 -0.000002
TS 18
MIN 39 <--> CH2O+C2HNO
E= -320.6995010500 ZPE= 34.2596000000
O 1.878996 0.915256 0.000428
C 1.901475 -0.399877 -0.000381
H 0.764716 1.121304 -0.001240
H 2.228121 -0.900012 -0.919182
H 2.229770 -0.900855 0.917327
C -0.384649 0.206572 -0.000291
O 0.284983 -0.859471 0.000466
C -1.806123 0.076683 -0.000048
N -2.971237 0.133287 0.000037
TS 19
CO+C2H3NO <--> CH2O+C2HNO

E= -320.6961103500 ZPE= 33.0357700000
O -1.510880 1.117614 -0.000302
C -1.629599 -0.165876 0.000564
H -1.956757 -0.652819 0.928311
H -1.957859 -0.653997 -0.926170
H -0.191050 1.310971 -0.001470
C 0.880061 0.700488 -0.000669
O 2.029456 0.858848 0.000583
C 0.106768 -0.875429 -0.000031
N 0.544812 -1.967278 -0.000300
TS 20
MIN 27 <--> MIN 27
E= -320.6976907400 ZPE= 34.4053800000
O 1.644971 1.051847 0.158133
C -2.642872 -0.000030 0.292187
H -3.141044 0.945141 0.480706
H -3.140920 -0.945259 0.480721
H 2.373794 -0.000314 0.428235
C 0.952214 0.000072 -0.087489
O 1.644481 -1.052087 0.157928
C -0.353102 0.000254 -0.681265
N -1.449270 0.000082 -0.151249
TS 21
MIN 29 <--> CO+C2H3NO
E= -320.6969184100 ZPE= 34.7925600000
O 0.242151 1.593567 0.036163
C 2.243340 -0.774459 0.103983
H 2.807852 -1.522904 -0.447367
H 0.995796 1.801684 -0.551964
H 2.717265 -0.300810 0.968600
C -1.628551 -0.192754 -0.395050
O -2.507250 -0.616521 0.225737
C 0.108096 0.277477 0.232793
N 1.037511 -0.522275 -0.244975
TS 22
CO2+C2H3N <--> CO2+C2H3N
E= -320.6927267900 ZPE= 32.4121100000
O -1.858238 1.180205 -0.291117
C 2.335034 0.584617 0.478766
H 2.530387 1.537920 -0.000586
H 3.190230 -0.316672 -0.429338
H 2.799428 0.345191 1.429403
C -2.005186 0.056297 -0.000229
O -2.202002 -1.058594 0.290529
C 1.142780 -0.218132 0.032172
N 2.160873 -0.725146 -0.579861
TS 23
MIN 34 <--> MIN 37
E= -320.6983741100 ZPE= 36.0029700000
O -1.183084 -1.305931 -0.287625
C -1.481575 1.110543 -0.171683
H -2.388397 0.995676 -0.765213
H -0.779480 1.786774 -0.669553
H -1.716545 1.547361 0.804502
C -0.836497 -0.219077 0.033263
O 0.402747 -0.079727 0.844978

C 2.463219 0.172869 -0.564425
N 1.465177 0.052777 0.055501
TS 24
 MIN 10 <--> HNC+C2H2O2
E= -320.6927280400 ZPE= 33.2699400000
O 2.055137 -0.500060 0.000000
C 0.057851 -0.999557 0.000000
H -0.095448 -1.542184 0.927607
H -0.095448 -1.542184 -0.927607
H -0.737149 1.051145 0.000000
C 0.988743 0.152261 0.000000
O 0.639047 1.348675 0.000000
C -2.630802 -0.283358 0.000000
N -1.588597 0.289747 0.000000
TS 25
 MIN 30 <--> CO2+C2H3N
E= -320.6934234300 ZPE= 33.7651500000
O -1.837729 -0.894882 -0.166247
C 2.588733 0.167750 -0.131114
H 3.004596 0.125962 -1.134170
H 3.184744 0.528679 0.702729
H -0.683634 -1.505094 0.188388
C -1.125250 0.177354 0.022574
O -1.353063 1.361666 0.005109
C 0.243309 -0.578614 0.281949
N 1.397125 -0.211824 0.070244
TS 26
 HCN+CH2O+CO <--> CN+CO+CH3O
E= -320.6905206200 ZPE= 32.0876200000
O -1.624450 -0.546226 -0.432653
C -0.969105 -0.996383 0.528931
H -0.460273 -0.294706 1.200120
H -1.004661 -2.073786 0.680423
H -1.431765 0.556511 -0.529531
C 1.954134 -0.163207 -0.182753
O 1.272699 -1.094177 -0.186157
C -0.413748 1.892308 -0.331657
N 0.326147 1.505557 0.501763
TS 27
 MIN 11 <--> MIN 24
E= -320.6937575100 ZPE= 35.7022100000
O -0.345604 1.418517 -0.123992
C -0.999469 -0.870828 -0.393332
H -0.575727 -1.864320 -0.173829
H -1.377792 -0.874115 -1.436236
H -1.347303 1.237354 0.032960
C 0.049907 0.188840 -0.190214
O -1.843072 -0.349429 0.563793
C 1.437017 -0.065989 0.052478
N 2.555073 -0.366252 0.177871
TS 28
 MIN 4 <--> MIN 44
E= -320.6927511500 ZPE= 35.6742300000
O 0.356481 1.389102 -0.009335
C 2.103360 -0.423906 -0.071536
H 1.299690 1.243654 -0.407754

H 2.693769 -1.312342 -0.256646
H 2.420359 0.201057 0.764049
C -0.104641 0.166690 0.053364
O 0.758188 -0.800224 0.021894
C -1.486215 -0.131007 -0.005446
N -2.629457 -0.359150 -0.008344
TS 29
MIN 2 <--> HOCN+C2H2O
E= -320.6905211300 ZPE= 34.8863400000
O -0.226673 -1.151596 -0.000029
C 0.052656 1.068412 -0.000021
H -0.643532 -2.035816 0.000023
H 0.064498 1.698036 -0.895856
H 0.064492 1.698086 0.895778
C 1.207153 0.207181 0.000003
O 2.302339 -0.147461 0.000024
C -1.175785 0.073741 0.000000
N -2.370704 0.133735 0.000029
TS 30
CH2O+C2HNO <--> CH2O+C2HNO
E= -320.6891139000 ZPE= 34.2462700000
O 1.677174 0.543422 0.000390
C 2.865802 0.286048 -0.000257
H 3.237030 -0.754057 -0.001128
H 3.616869 1.093495 0.000008
H 0.402165 -0.632469 0.000204
C -1.515628 -1.087995 -0.000054
O -0.249220 -1.388093 0.000100
C -1.793804 0.341303 -0.000058
N -2.288275 1.402038 -0.000113
TS 31
MIN 17 <--> MIN 17
E= -320.6906456200 ZPE= 35.6172800000
O 0.445727 1.101753 -0.013837
C 2.266517 -0.000016 0.015393
H 2.529360 -0.918295 -0.490608
H 2.338695 -0.000318 1.094699
H 2.529392 0.918531 -0.490100
C -0.153390 0.000013 -0.010857
O 0.445750 -1.101718 -0.013837
C -2.728200 -0.000022 0.010747
N -1.548403 -0.000007 0.002243
TS 32
MIN 23 <--> HOCN+C2H2O
E= -320.6858262400 ZPE= 32.8474700000
O -1.489302 -1.143588 -0.235607
C -1.579006 1.351922 0.053457
H -0.436246 -1.387599 -0.202537
H -2.339980 1.779720 -0.595713
H -0.997230 1.989321 0.708479
C -1.353257 0.075596 -0.015216
O 0.589632 -0.592966 0.456695
C 1.665677 -0.054310 0.049214
N 2.652905 0.467390 -0.314809
TS 33
MIN 27 <--> MIN 29

E= -320.6899938000 ZPE= 35.6399700000
O -2.249470 -0.685971 -0.159487
C 2.458224 -0.058847 -0.166035
H 2.579693 1.017407 -0.291896
H 3.315781 -0.712901 -0.288812
H -0.860868 1.794579 0.716686
C -1.147591 -0.298957 -0.002032
O -0.621536 1.349115 -0.114054
C 0.134013 -0.198408 0.381916
N 1.323653 -0.580994 0.109895
TS 34
MIN 3 <--> MIN 21
E= -320.6898220600 ZPE= 35.6015800000
O 0.275218 -0.997547 0.000020
C -1.129559 -0.906724 -0.000013
H -1.515552 -1.392425 0.898802
H -1.515512 -1.392387 -0.898867
H 0.210713 1.776948 0.000003
C 1.011585 0.155197 -0.000002
O 2.204268 0.183627 -0.000007
C -0.834324 1.430474 0.000004
N -1.614535 0.492220 0.000003
TS 35
CH2O+C2HNO <--> CH2O+C2HNO
E= -320.6864612500 ZPE= 34.0854700000
O -1.972827 0.169275 -0.523653
C -2.391760 -0.627693 0.288103
H -1.790842 -0.927980 1.166697
H -3.393866 -1.086378 0.182921
H 0.379312 2.342578 0.239413
C 0.734626 0.546682 0.572536
O 0.924676 1.631206 -0.136335
C 1.502013 -0.546258 0.017611
N 2.017332 -1.566923 -0.225518
TS 36
CO2+C2H3N <--> CO2+C2H3N
E= -320.6758613700 ZPE= 27.6787500000
O -1.916275 0.999652 -0.499245
C 1.035401 0.218545 0.817729
H 1.223211 2.554649 0.436713
H 0.571023 2.231625 0.242316
H 1.324830 0.576031 1.815923
C -1.943532 -0.109990 -0.129549
O -2.006052 -1.219992 0.231088
C 2.144438 -0.120032 0.055825
N 2.977387 -0.504388 -0.687675
TS 37
MIN 9 <--> HCN+CH2O+CO
E= -320.6829837400 ZPE= 33.4318900000
O -1.483965 0.506467 0.000000
C -1.899517 -0.680974 0.000000
H -2.166420 -1.176728 -0.942500
H -2.166420 -1.176729 0.942500
H -0.226303 -1.429012 0.000000
C 0.402279 0.678299 0.000000
O 0.884742 1.721583 0.000000

C 0.788496 -0.904392 0.000000
N 1.943626 -1.228503 0.000000
TS 38
HCN+C2H2O2 <--> HNC+C2H2O2
E= -320.6802208700 ZPE= 31.9531400000
O -0.003610 0.863201 -0.151453
C -2.481904 0.167708 0.033623
H 1.722662 0.126122 -0.181984
H -2.999328 0.342720 0.972714
H -3.082031 0.143039 -0.871640
C -1.038840 0.264247 -0.041425
O -1.458787 -0.980713 0.111773
C 2.726795 -0.476726 -0.513344
N 2.974509 0.085263 0.503603
TS 39
CO2+C2H3N <--> CO+C2H3NO
E= -320.6798206300 ZPE= 32.8068900000
O 0.878454 0.050685 -0.797478
C -1.069167 1.011494 0.125384
H -0.615539 1.307874 1.063891
H -1.074346 1.733482 -0.681993
H 0.125593 -0.551613 -0.593902
C 2.065018 -0.368528 -0.294765
O 2.629695 -0.137864 0.708518
C -2.067676 0.028360 0.148920
N -2.867135 -0.831467 0.149493
TS 40
HNC+CH2O+CO <--> HNC+CH2O+CO
E= -320.6723318800 ZPE= 29.9295100000
O 0.951143 -1.396319 -0.000098
C 2.114538 -0.864735 0.000102
H 2.878598 -1.655645 0.000199
H 1.903743 0.482488 0.000115
H 0.263722 -0.678772 -0.000183
C -3.034490 -0.124392 0.000140
O -1.995793 -0.592504 -0.000071
C 0.183275 2.220920 -0.000069
N 1.104457 1.481679 0.000026
TS 41
MIN 9 <--> CO+C2H3NO
E= -320.6803176300 ZPE= 34.9830300000
O 0.730812 -0.384799 0.578044
C 1.832326 -0.730103 -0.278821
H 1.491659 -0.959581 -1.296571
H 2.317735 -1.610247 0.149101
H 2.536380 0.105919 -0.311449
C -1.085939 -0.229063 0.044939
O -1.880795 -1.034008 -0.161027
C -0.205849 0.877801 0.102248
N -0.055591 2.043222 -0.155345
TS 42
CO+C2H3NO <--> CO+C2H3NO
E= -320.6747393500 ZPE= 32.0674800000
O -2.824475 -0.423837 -0.000028
C -0.943193 1.238446 0.000005
H 0.154026 1.204694 0.000035

H -1.286711 1.741874 0.908558
H -1.286662 1.741855 -0.908576
C 3.713412 -0.456451 -0.000029
O 2.825397 0.255334 0.000011
C -1.603303 -0.151375 0.000002
N -0.655647 -1.017732 0.000037
TS 43
MIN 12 <--> HCN+C2H2O2
E= -320.6773436500 ZPE= 34.0907900000
O -0.061018 -1.669924 -0.149633
C 0.061725 -0.487262 0.503743
H -0.096108 -1.523547 -1.109258
H 0.504827 1.548866 0.590588
H 0.190533 -0.694253 1.573273
C -1.124927 0.576356 0.376062
O -1.977638 0.691282 -0.414170
C 1.119866 0.633509 0.151148
N 2.195716 0.594636 -0.389985
TS 44
CH2O+C2HNO <--> HCN+CH2O+CO
E= -320.6699713000 ZPE= 30.7526400000
O -1.145333 -1.299599 -0.000044
C -2.207122 -0.696155 0.000053
H 0.355601 -0.501159 -0.000154
H -2.231623 0.405127 0.000060
H -3.155609 -1.257949 0.000138
C 1.529376 -0.647425 -0.000077
O 2.656592 -0.495649 0.000082
C 0.124589 1.306155 -0.000054
N -0.534214 2.277216 0.000018
TS 45
CO+C2H3NO <--> CO+C2H3NO
E= -320.6726249900 ZPE= 32.5741700000
O -2.311346 -0.028304 -0.645423
C -0.931218 1.242591 0.417242
H -1.581196 1.929482 -0.103715
H 0.093032 1.168542 0.072900
H -1.097864 1.114984 1.479949
C 3.118510 -0.473336 -0.154163
O 2.498537 0.481748 -0.177240
C -1.386042 -0.623028 -0.032409
N -0.531286 -1.245417 0.535449
TS 46
MIN 11 <--> MIN 24
E= -320.6762914100 ZPE= 35.2386700000
O -1.590274 -0.758966 -0.707590
C -1.624470 -0.510108 0.504452
H -1.294393 -1.242439 1.260551
H -2.226926 0.327330 0.907488
H -0.469599 2.274288 0.059245
C 0.228980 0.574767 0.425236
O 0.246845 1.693783 -0.251491
C 1.310646 -0.292395 0.039061
N 2.178203 -1.067330 -0.052447
TS 47
MIN 1 <--> CO+C2H3NO

E= -320.6732406200 ZPE= 33.9882300000
O 1.478330 -1.533209 0.127565
C 1.080282 1.587310 0.321331
H 0.136614 1.965140 0.686765
H 1.423171 1.993609 -0.619939
H 1.837887 1.453774 1.085796
C 1.500241 -0.412396 -0.107719
O -2.379842 -0.370188 0.418323
C -1.425663 0.006572 -0.188479
N -0.444962 0.389392 -0.810075
TS 48
MIN 44 <--> CH2O+C2HNO
E= -320.6726769800 ZPE= 35.3265800000
O 0.150063 1.517898 0.235545
C 2.016793 -0.585102 0.255418
H 2.803709 -1.345990 0.246866
H 2.191256 0.384566 0.740381
H 0.629319 2.162171 -0.306016
C -0.259330 0.519930 -0.585507
O 0.941705 -0.828650 -0.289796
C -1.383712 -0.188449 -0.018998
N -2.371562 -0.741858 0.263900
TS 49
MIN 48 <--> MIN 49
E= -320.6744314400 ZPE= 36.4697400000
O -1.026833 1.279357 -0.007959
C -1.551660 0.021513 -0.109042
H -0.823564 1.506690 0.909944
H -1.942560 -0.110043 -1.117259
H -2.298828 -0.221421 0.650793
C 0.698208 -1.206010 0.069810
O -0.593069 -1.141964 0.046847
C 2.269432 0.786118 -0.067698
N 1.361184 0.016558 -0.016143
TS 50
MIN 43 <--> HNC+CH2O+CO
E= -320.6709368300 ZPE= 34.4954900000
O 1.343991 0.883670 -0.416233
C 1.370600 -0.071348 0.444349
H 2.234868 -0.724532 0.391850
H 0.472602 1.405464 -0.317024
H 0.828765 0.040614 1.382840
C -1.067523 -1.374063 -0.234992
O 0.134661 -1.447104 -0.120396
C -1.511812 0.375961 0.281521
N -1.159005 1.457518 -0.015701
TS 51
MIN 9 <--> MIN 28
E= -320.6706515100 ZPE= 34.6010100000
O 0.019962 -1.080906 0.000008
C -1.329606 -1.005188 0.000000
H -2.122852 0.856989 -0.000216
H -1.791333 -1.317423 0.935023
H -1.791360 -1.317446 -0.935003
C 0.868851 0.043101 -0.000002
O 2.051863 -0.062718 -0.000009

C 0.028663 1.349049 -0.000005
N -1.182358 1.229300 0.000035
TS 52
 MIN 14 <--> CO+C2H3NO
E= -320.6681946200 ZPE= 33.5413900000
O -1.837593 -0.735516 -0.254237
C -1.613275 0.281478 0.247632
H 1.389431 1.683830 -0.963817
H -1.177546 1.116114 0.784348
H 1.005490 0.997056 1.495331
C 0.618096 0.634697 0.541066
O 0.555471 1.617873 -0.475514
C 1.037135 -0.664666 0.161175
N 1.255409 -1.766416 -0.168156
TS 53
 CH2O+C2HNO <--> HCN+CH2O+CO
E= -320.6655533900 ZPE= 31.9680100000
O -0.992091 -1.215079 0.251229
C -0.118246 -1.951573 -0.182746
H -0.193970 0.902878 1.212699
H -0.326704 -3.029055 -0.298175
H 0.875940 -1.564027 -0.454455
C -0.911232 1.049447 0.402035
O -1.497550 1.457964 -0.487228
C 1.453390 0.796879 0.257666
N 2.431199 0.339800 -0.204830
TS 54
 MIN 52 <--> MIN 52
E= -320.6715596300 ZPE= 35.9768100000
O -1.951546 -0.591647 0.000000
C -0.718272 1.452882 0.000000
H -1.625548 2.041204 0.000000
H -1.753275 -1.539708 0.000000
H 0.242577 1.945999 0.000000
C -0.816900 0.129955 0.000000
O 0.264965 -0.787589 0.000000
C 2.594027 0.120485 0.000000
N 1.467965 -0.233362 0.000000
TS 55
 MIN 44 <--> MIN 44
E= -320.6701908700 ZPE= 35.3951500000
O 0.161582 1.723853 -0.102519
C -2.177307 -0.770336 0.007701
H 0.623104 2.122173 0.650829
H -2.204279 -1.852255 0.000490
H -3.047811 -0.127880 -0.016176
C 0.126090 0.359128 0.019760
O -1.019976 -0.203407 0.013251
C 1.299476 -0.418468 -0.011595
N 2.286656 -1.046793 -0.002314
TS 56
 MIN 43 <--> HCN+CH2O+CO
E= -320.6650304200 ZPE= 32.5952500000
O 0.955263 -1.247936 -0.345459
C 1.679504 -0.436836 0.319724
H 1.504759 -0.280379 1.385762

H -0.089857 -1.039751 -0.146650
H 2.641207 -0.161097 -0.107745
C -0.448695 1.374154 -0.173046
O 0.739517 1.330163 -0.033713
C -1.329546 -0.173981 -0.026768
N -2.431704 -0.536659 0.168936
TS 57
 CO+C2H3NO <--> CH2O+C2HNO
E= -320.6645109100 ZPE= 32.3487600000
O 1.573841 -0.685361 -0.280737
C 0.639285 -1.335049 0.268824
H 0.459408 -1.250555 1.346508
H 1.388176 0.468431 -0.108000
H 0.191085 -2.172213 -0.267367
C -0.453978 1.410016 0.126722
O 0.769283 1.500909 0.006060
C -1.139190 0.007319 -0.012170
N -2.151480 -0.580538 -0.153427
TS 58
 MIN 9 <--> CO2+C2H3N
E= -320.6658453300 ZPE= 33.9392600000
O -0.546785 -1.294935 0.000000
C 1.879275 -0.849198 0.000000
H 1.594480 -1.332209 -0.925164
H 1.594480 -1.332209 0.925165
H 2.683036 -0.127784 0.000000
C -0.987705 -0.113586 0.000000
O -2.097172 0.382382 0.000000
C 0.251667 0.848870 0.000000
N 1.202891 1.539445 0.000000
TS 59
 HCN+C2H2O2 <--> HCN+C2H2O2
E= -320.6589470800 ZPE= 30.1366700000
O 0.166282 1.574312 -0.411169
C 0.916868 0.925430 0.387172
H -1.106508 0.892585 -0.304531
H -0.473033 -0.551425 0.391806
H 1.063160 1.218284 1.438109
C 1.209477 -0.425258 0.115986
O 1.812361 -1.373176 -0.211406
C -1.604489 -0.164009 0.017703
N -2.634843 -0.740788 0.047150
TS 60
 MIN 20 <--> HNC+CH2+CO2  (Note that the IRCs computed using dft and mp2 differ in the products obtained from this ts. See below)
E= -320.6594999800 ZPE= 31.0079100000
O -1.389721 -0.406574 0.000000
C -0.347789 -1.966872 -0.000001
H -0.847706 -2.369406 0.889811
H 0.902600 -1.132169 0.000003
H -0.847701 -2.369404 -0.889816
C -1.049389 0.731438 0.000000
O -0.841439 1.867699 0.000000
C 2.521096 0.577864 -0.000003
N 1.699796 -0.267515 0.000004
TS 61

MIN 24 <--> MIN 50
E= -320.6667305800 ZPE= 35.7672100000
O -1.133140 0.642605 -0.321397
C -0.227238 1.609336 0.247922
H -0.351368 1.669023 1.323103
H -0.197245 2.524694 -0.332653
H -1.813861 -1.506876 0.286971
C -0.346735 -0.404598 -0.175775
O -0.849531 -1.570979 0.174547
C 1.042367 -0.047597 -0.049449
N 2.201925 -0.314670 -0.034115
TS 62
MIN 24 <--> MIN 44
E= -320.6662692700 ZPE= 35.5209000000
O -0.813203 -0.758419 -0.494483
C -1.923961 -0.522596 0.344105
H -2.874424 -0.628243 -0.163557
H -1.190797 1.645416 0.092439
H -1.781700 -0.884375 1.352595
C 0.002329 0.190502 -0.051633
O -0.235259 1.520532 -0.035259
C 1.379582 -0.157215 0.039073
N 2.498131 -0.470549 0.138169
TS 63
MIN 13 <--> HOCN+C2H2O
E= -320.6639623700 ZPE= 34.3001500000
O 1.054773 1.070706 -0.132450
C -0.978213 1.260008 0.091037
H -0.985695 1.759190 1.054544
H -1.160394 1.856200 -0.796741
H 1.932177 1.327015 0.227720
C -0.802799 -0.198374 -0.001587
O -1.602385 -1.098463 -0.046269
C 0.756727 -0.356618 -0.021609
N 1.534358 -1.278636 0.076740
TS 64
MIN 4 <--> MIN 6
E= -320.6598985100 ZPE= 32.4476300000
O -0.462045 -0.869189 0.000179
C -3.177207 -0.219691 -0.000046
H -1.457292 -0.614258 0.000214
H -4.085886 -0.848940 -0.001137
H -3.528227 0.827913 0.000775
C 0.298773 0.209609 0.000020
O -0.062337 1.368833 -0.000048
C 1.734503 -0.139778 -0.000038
N 2.875721 -0.351816 -0.000074
TS 65
MIN 4 <--> MIN 4
E= -320.6596465900 ZPE= 32.5770800000
O -0.237523 -1.249413 -0.148138
C -2.987613 0.147757 0.159269
H -3.971790 0.100878 -0.339179
H -3.069938 -0.487818 1.058842
H -1.420899 0.750144 -0.202424
C 0.244224 -0.129882 -0.094684

O -0.415764 1.005972 -0.148535
C 1.699417 0.062330 0.050998
N 2.850393 0.157584 0.166093
TS 66
MIN 4 <--> MIN 4
E= -320.6614911900 ZPE= 34.3087600000
O -0.408976 1.126333 0.000000
C -2.658672 0.000000 0.000001
H -3.750384 0.000000 0.000001
H -2.127312 0.000000 -0.933986
H -2.127312 0.000000 0.933987
C 0.159598 0.000000 0.000000
O -0.408976 -1.126333 0.000000
C 1.646687 0.000000 0.000000
N 2.808992 0.000000 0.000000
TS 67
MIN 9 <--> CO2+C2H3N
E= -320.6608386500 ZPE= 34.4584500000
O -2.179734 0.145880 0.000000
C 2.086186 -0.726204 0.000000
H 1.582578 -0.604770 -0.940657
H 1.582580 -0.604770 0.940658
H 3.115262 -1.086917 -0.000001
C -0.997787 -0.150878 0.000000
O -0.401849 -1.274112 0.000000
C 0.056838 0.958668 0.000000
N 1.071546 1.547543 0.000000
TS 68
MIN 26 <--> MIN 26
E= -320.6571483800 ZPE= 32.3955400000
O -0.033908 -1.309256 -0.000186
C -2.676000 -0.407851 0.000058
H -3.022658 0.640609 0.000069
H -0.993213 -0.953320 -0.000346
H -3.585575 -1.034986 0.000579
C 0.892115 -0.367009 -0.000012
O 2.084726 -0.558138 0.000177
C 0.361374 1.023255 -0.000040
N -0.038576 2.113783 -0.000038
TS 69
MIN 20 <--> CO2+C2H3N
E= -320.6585697000 ZPE= 33.5286900000
O 0.693933 -1.220249 0.000504
C -1.359230 -1.501749 -0.000328
H -1.734109 -1.083281 -0.923532
H -1.734410 -1.083733 0.922986
H -0.961438 -2.508101 -0.000522
C 1.174302 -0.122499 0.000069
O 1.894192 0.784287 -0.000342
C -1.442641 1.953909 0.000235
N -0.929948 0.883551 -0.000012
TS 70
CO2+C2H3N <--> H2+CO2+C2HN
E= -320.6499919500 ZPE= 28.4677600000
O -1.899704 -1.222653 0.294898
C 1.122945 0.363738 0.715130

H 1.481155 0.610473 1.730475
H 1.341541 2.415612 0.410855
H 0.789595 1.887981 0.240904
C -1.950983 -0.123689 -0.100587
O -2.036631 0.971438 -0.503184
C 2.960065 -0.605570 -0.730377
N 2.155176 -0.101603 -0.002992
TS 71
MIN 4 <--> MIN 5
E= -320.6552115900 ZPE= 32.2039400000
O -0.000355 1.453307 0.000197
C 3.195701 -0.301093 -0.010837
H 4.025446 -0.967348 0.254146
H 3.568277 0.732176 0.204467
H 1.477426 -0.605695 -0.042783
C -0.313492 0.288593 -0.072468
O 0.468530 -0.784544 -0.061541
C -1.716944 -0.166342 0.035810
N -2.829735 -0.490884 0.051413
TS 72
MIN 31 <--> MIN 46
E= -320.6598150400 ZPE= 35.1588700000
O -1.259579 0.261297 0.570930
C -1.655239 -0.487625 -0.656706
H -1.354711 0.138416 -1.494152
H -2.730355 -0.609130 -0.568122
H -1.101172 -1.424239 -0.612908
C -0.197565 0.636845 1.037566
O 1.047468 0.988293 -0.676930
C 1.333595 -0.123806 -0.202094
N 1.428339 -1.179179 0.350084
TS 73
CO2+C2H3N <--> CO2+C2H3N
E= -320.6526630100 ZPE= 31.4318500000
O -1.005417 -1.242726 -0.000119
C 0.917772 1.245903 -0.000097
H 2.623148 0.839599 0.000017
H 1.029197 1.813979 0.922380
H 1.029195 1.813767 -0.922703
C -1.662101 -0.273307 -0.000003
O -2.381697 0.649622 0.000116
C 2.308547 -1.041651 0.000115
N 1.861438 0.098832 0.000035
TS 74
MIN 51 <--> CO+C2H3NO
E= -320.6573187800 ZPE= 34.7827100000
O 1.188310 0.457567 0.000007
C 2.623815 0.325813 -0.000006
H 2.988608 1.353580 0.000006
H 2.958628 -0.199192 0.898704
H 2.958614 -0.199167 -0.898735
C -1.823805 0.374195 0.000013
O -2.968981 0.376668 -0.000010
C -0.593314 -1.077653 0.000003
N 0.585620 -0.766176 -0.000002
TS 75

H2+CO+C2HNO <--> H2+CO+C2HNO
E= -320.6409431100 ZPE= 24.7033600000
O 0.796293 1.971807 -0.000017
C 0.637403 0.838837 -0.000017
H 4.253977 -0.166316 0.000109
H 4.010842 -0.869254 0.000100
H 1.100598 -0.400675 -0.000028
C -0.504684 -1.558893 -0.000004
O 0.720255 -1.593846 -0.000025
C -1.169229 -0.116089 0.000011
N -2.182677 0.489918 0.000030
TS 76
CH2O+C2HNO <--> HOCH+C2HNO
E= -320.6488985400 ZPE= 31.0650800000
O -2.365222 0.258603 -0.000094
C -1.998239 -0.959300 0.000126
H -1.463271 0.837069 0.000050
H -2.867824 -1.645025 -0.000263
H -0.620080 -0.959104 0.000159
C 0.489788 -0.005274 -0.000017
O -0.035265 1.135527 0.000055
C 1.950194 -0.103266 -0.000013
N 3.072087 -0.425563 -0.000029
TS 77
MIN 9 <--> MIN 26
E= -320.6475063200 ZPE= 30.2235500000
O 1.986727 -0.700002 0.105243
C -2.522883 -0.334072 -0.003028
H -1.228591 -0.804047 -0.302878
H -3.308334 -0.997351 0.387998
H -2.723643 0.699095 0.314626
C 0.815702 -0.408545 -0.005041
O -0.184248 -1.252197 -0.105878
C 0.414306 1.028869 -0.026306
N 0.085426 2.143198 -0.026917
TS 78
MIN 4 <--> MIN 40
E= -320.6560006900 ZPE= 35.6196600000
O 1.232511 -0.766425 -0.069707
C 2.201854 0.297136 0.270317
H 1.900492 0.766842 1.206557
H 2.242023 1.030413 -0.535256
H 3.147121 -0.229139 0.373591
C 0.018311 -0.447202 -0.355770
O -0.356929 0.831713 -0.271544
C -1.519515 -0.020135 -0.012006
N -2.642600 -0.152746 0.324267
TS 79
CH2O+C2HNO <--> CH2O+C2HNO
E= -320.6525224600 ZPE= 33.7512700000
O 1.344777 -0.477267 0.255055
C 2.561683 -0.151651 -0.102474
H 3.118006 0.413079 0.632400
H 2.882402 -0.251403 -1.133207
H 0.854673 -1.010381 -0.392600
C -0.688573 0.716872 -0.082614

O -0.878082 1.891217 0.006334
C -1.571250 -0.440406 0.008278
N -1.771401 -1.601684 -0.019549
TS 80
MIN 9 <--> MIN 9
E= -320.6533266500 ZPE= 34.5690200000
O 0.346132 -0.226438 0.000043
C -0.375350 -1.634119 -0.000011
H -1.416672 -1.239531 -0.000017
H -0.022519 -2.097797 0.918124
H -0.022489 -2.097748 -0.918159
C 1.467238 0.175583 0.000004
O 2.493161 0.698117 -0.000021
C -1.834918 1.361344 0.000010
N -2.399213 0.320686 -0.000021
TS 81
MIN 4 <--> MIN 58
E= -320.6504908200 ZPE= 32.9487200000
O -0.834082 0.057419 -0.711630
C -2.494770 -0.750635 0.392926
H -1.927901 -0.996287 1.314635
H -2.517662 -1.705728 -0.166871
H -1.601350 0.676829 -0.642024
C 0.253866 0.569943 -0.086941
O 0.353913 1.689258 0.340470
C 1.321187 -0.431192 -0.001217
N 2.200938 -1.182418 0.090705
TS 82
H2+C3HNO2 <--> H2+C3HNO2
E= -320.6442468600 ZPE= 29.1459700000
O 1.935925 -1.145878 -0.135736
C 1.109393 -0.337486 0.117813
H 1.237186 0.499309 1.192849
H 0.578621 1.895272 0.764187
H 1.149799 1.528704 1.479065
C -0.088506 0.348375 -0.300177
O -0.003680 1.636980 -0.288934
C -1.340880 -0.313473 0.003260
N -2.357658 -0.862371 0.147984
TS 83
H2+C3HNO2 <--> H2+C3HNO2
E= -320.6406418200 ZPE= 28.1130900000
O -1.884413 0.652502 -0.116886
C -1.589658 -0.488630 -0.306943
H -0.906278 4.089012 0.601318
H -1.204790 3.421105 0.468559
H -2.179477 -1.274344 -0.785525
C 0.641544 -0.611732 0.816595
O -0.387816 -1.052779 0.091222
C 1.650006 -0.001251 -0.005060
N 2.608146 0.510875 -0.443799
TS 84
MIN 20 <--> MIN 20
E= -320.6496682000 ZPE= 34.3623600000
O 1.605559 -0.233319 -0.133397
C 0.754432 -1.593219 0.100237

H 1.008395 -2.148312 -0.804151
H -0.305753 -1.292257 0.178246
H 1.225587 -1.982086 1.010311
C 1.046407 0.863419 -0.047119
O 0.232187 1.676016 0.095867
C -2.616231 -0.524656 -0.058382
N -1.676834 0.201117 -0.007512
TS 85
MIN 46 <--> CO+C2H3NO
E= -320.6469633300 ZPE= 33.3444000000
O -1.161176 0.867965 -0.170651
C -1.694664 -1.025832 0.193319
H -2.686995 -0.598705 0.232551
H -1.181022 -1.255236 1.117235
H -1.372147 -1.565783 -0.686727
C -0.324052 1.688888 -0.098251
O 1.540551 0.747530 0.220648
C 1.298274 -0.439061 -0.002121
N 0.932546 -1.549744 -0.231531
TS 86
MIN 26 <--> CH2+C2HNO2
E= -320.6460934700 ZPE= 32.8377900000
O -0.846093 -0.039481 -0.674700
C -2.503013 -0.871088 0.394702
H -0.819591 -1.021783 -0.707681
H -3.256506 -0.292267 -0.174067
H -2.367888 -0.277044 1.321344
C 0.244034 0.536267 -0.104244
O 0.269249 1.687816 0.228190
C 1.395694 -0.364980 0.039687
N 2.319778 -1.056682 0.164517
TS 87
CH2O+C2HNO <--> CH2O+C2HNO
E= -320.6459607300 ZPE= 32.8623800000
O 2.007434 -0.744296 -0.000053
C 2.768592 0.226340 0.000087
H 3.844608 0.035827 0.000134
H 2.348671 1.237886 0.000160
H 0.945256 -0.402102 -0.000065
C -0.680172 -0.234032 -0.000007
O 0.036146 0.816975 -0.000093
C -2.144222 -0.045350 0.000016
N -3.307480 -0.162114 0.000053
TS 88
MIN 4 <--> H2+C3HNO2
E= -320.6412693900 ZPE= 30.5374200000
O -0.758873 -0.715712 0.122300
C -2.018680 -0.558349 -0.372693
H -2.533537 -1.460876 0.011769
H -2.776250 0.540322 0.432110
H -2.966323 0.343103 1.177357
C 0.121518 0.339787 -0.011911
O -0.187592 1.493841 -0.084265
C 1.496828 -0.151300 0.024573
N 2.607119 -0.489772 0.033524
TS 89

MIN 4 <--> H2+C3HNO2
E= -320.6407594900 ZPE= 30.5430300000
O 0.751048 -0.765074 -0.034280
C 2.076420 -0.607045 -0.301077
H 2.736278 0.179022 1.435476
H 2.225895 0.442888 -0.632112
H 2.843058 -0.511309 1.060743
C -0.117308 0.327067 -0.024773
O 0.211093 1.478371 -0.036992
C -1.498499 -0.138645 0.028601
N -2.609434 -0.472177 0.069938
TS 90
MIN 9 <--> H2+C3HNO2
E= -320.6412045600 ZPE= 30.9047500000
O 1.180921 0.426570 -0.110837
C 1.562740 -0.873931 -0.265964
H 2.165210 -1.293990 1.461337
H 2.645238 -0.815470 -0.466048
H 1.558291 -1.584331 0.996271
C -0.176507 0.660909 -0.002712
O -0.605907 1.769812 0.118718
C -1.034698 -0.533455 -0.039407
N -1.868294 -1.342629 -0.029444
TS 91
MIN 11 <--> CH2O+C2HNO
E= -320.6447221600 ZPE= 33.5005700000
O 2.188874 0.191147 0.313172
C 2.160763 -0.976515 -0.197096
H 1.255828 -1.574028 -0.108196
H 3.053094 -1.293982 -0.729604
H 1.245605 0.405263 0.601587
C -0.497360 0.284406 0.033441
O -0.177349 1.440176 -0.230875
C -1.898463 -0.163909 0.012739
N -2.890910 -0.778818 0.069047
TS 92
MIN 20 <--> CO2+C2H3N
E= -320.6445296700 ZPE= 34.2732100000
O -0.272944 -1.248755 0.000000
C 2.072272 -0.635676 0.000000
H 3.068181 -1.081307 0.000001
H 1.593712 -0.465553 0.944539
H 1.593713 -0.465554 -0.944539
C -0.958256 -0.192520 0.000000
O -2.136705 0.057942 0.000000
C 1.055249 1.556665 0.000000
N 0.000857 1.024015 0.000000
TS 93
H2+CO+C2HNO <--> HNC+H2+2CO
E= -320.6303644000 ZPE= 25.8106300000
O -3.315628 0.302899 -0.000370
C -2.234430 0.667356 0.000000
H -0.140029 1.627573 0.000758
H -1.196817 1.478182 0.000429
H -0.102980 0.691519 0.000619
C 3.883172 -0.162563 -0.000498

O 3.092555 0.655565 0.000163
C -0.396562 -1.744262 0.000158
N -0.612667 -0.575452 0.000271
TS 94
MIN 9 <--> H2+C3HNO2
E= -320.6360319300 ZPE= 30.4358800000
O -1.196815 0.431189 -0.011175
C -1.755178 -0.758353 -0.335084
H -2.239711 -1.437197 0.913117
H -1.652447 -1.748135 1.369905
H -0.951123 -1.468013 -0.631732
C 0.172481 0.676737 0.013055
O 0.603257 1.788110 0.073724
C 1.041724 -0.512676 -0.022180
N 1.833941 -1.362185 -0.012348
TS 95
CH2O+C2HNO <--> HCN+C2H2O2
E= -320.6390285600 ZPE= 33.0771700000
O -1.177545 -0.956871 0.399555
C -2.017419 -0.573955 -0.339713
H 0.280304 0.744502 1.626345
H -1.179752 0.970211 -0.599330
H -2.677619 -0.077861 -1.026349
C 0.367800 0.619738 0.550651
O -0.315840 1.432041 -0.245244
C 1.473574 -0.102123 0.031773
N 2.368630 -0.728597 -0.384488
TS 96
MIN 45 <--> CH2O+C2HNO
E= -320.6405344000 ZPE= 34.0233000000
O -2.546131 -0.341861 -0.155193
C -2.211258 0.880933 0.086541
H -1.782210 -0.922054 0.147461
H -2.659629 1.639689 -0.548926
H -1.610322 1.140567 0.950062
C 1.012961 -0.873811 0.074263
O -0.152024 -0.467526 0.053921
C 2.115846 0.070318 -0.025099
N 3.161729 0.593179 -0.078949
TS 97
MIN 48 <--> HNC+CH2O+CO
E= -320.6396379000 ZPE= 33.6119800000
O -2.085377 -0.789366 -0.409585
C -1.176896 -0.519398 0.459620
H -2.985165 -0.534046 -0.136840
H -0.118506 -0.817969 0.236773
H -1.485884 -0.181352 1.449514
C 0.735544 1.552210 -0.167376
O -0.406249 1.375238 0.040561
C 2.677337 -0.969128 -0.059172
N 1.586665 -0.505102 0.000616
TS 98
MIN 7 <--> MIN 38
E= -320.6386887400 ZPE= 33.3156600000
O -0.713394 0.681040 0.000126
C -3.132629 0.106608 -0.000081

H -2.644282 -0.101335 0.935436
H -2.644193 -0.101023 -0.935620
H -4.176719 0.411510 -0.000084
C -0.489486 -0.498000 0.000062
O 0.859291 -0.956963 -0.000012
C 1.826088 -0.064199 -0.000028
N 2.724883 0.675969 -0.000051
TS 99
MIN 40 <--> CO+C2H3NO
E= -320.6375014600 ZPE= 32.8419200000
O 1.883272 -0.636030 0.000003
C 1.513859 1.470061 0.000001
H 0.980395 1.625722 0.927834
H 0.980343 1.625739 -0.927798
H 2.594655 1.468033 -0.000029
C 1.052150 -1.455462 0.000000
O -0.501017 -0.042233 -0.000009
C -1.748425 0.009368 -0.000001
N -2.931278 0.080401 0.000006
TS 100
MIN 17 <--> MIN 17
E= -320.6354771700 ZPE= 32.2347600000
O 0.415821 -0.884895 0.000022
C 3.119300 -0.194649 0.000010
H 3.446981 0.860423 0.000321
H 1.406988 -0.622788 0.000022
H 4.041730 -0.803640 -0.000329
C -0.336616 0.196765 -0.000004
O 0.021627 1.352602 -0.000032
C -2.863134 -0.356292 0.000004
N -1.701797 -0.150085 0.000000
TS 101
MIN 8 <--> MIN 36
E= -320.6388238300 ZPE= 34.5619900000
O 1.580555 -0.833938 0.081436
C 1.946380 0.955517 -0.113344
H 2.688184 0.642080 -0.845117
H 2.336207 1.271641 0.845180
H 1.192485 1.606489 -0.551692
C 0.570051 -0.228103 0.502446
O -0.567617 -0.558800 -0.383713
C -1.705361 -0.009018 -0.075743
N -2.740972 0.473046 0.155670
TS 102
MIN 7 <--> MIN 38
E= -320.6373827500 ZPE= 34.4991500000
O 0.857395 0.468380 0.827793
C 2.014879 0.366852 -0.595650
H 1.672438 -0.080285 -1.526811
H 2.928254 -0.046177 -0.188749
H 1.957221 1.453284 -0.617930
C 0.751565 -0.698715 0.377303
O -0.580672 -0.993382 -0.154347
C -1.501292 -0.062960 -0.130824
N -2.337516 0.748876 -0.137007
TS 103

MIN 35 <--> MIN 35
E= -320.6327549800 ZPE= 32.0800700000
O -2.042086 -0.615423 -0.000002
C 2.732330 -0.282376 0.000005
H 3.088445 0.763240 0.000190
H 1.054349 -0.831078 0.000015
H 3.638745 -0.914412 -0.000204
C -0.866671 -0.365215 0.000002
O 0.116545 -1.239931 0.000011
C -0.115111 2.130920 -0.000013
N -0.411500 0.989301 -0.000006
TS 104
H2+C3HNO2 <--> CH2O+C2HNO
E= -320.6279238800 ZPE= 30.7848400000
O 2.562022 0.391304 0.451876
C 1.852347 -0.176327 -0.306184
H 0.450778 -1.588827 0.449792
H 1.284574 -1.629877 0.291575
H 2.033031 -0.501673 -1.339024
C -0.613111 -0.412213 0.144885
O 0.258292 0.331987 -0.367924
C -1.975228 0.022255 0.054487
N -3.130706 0.190251 0.080987
TS 105
MIN 38 <--> CO+C2H3NO
E= -320.6337232100 ZPE= 34.9901400000
O -0.607602 0.113289 -0.234932
C -1.902556 -0.479996 0.106186
H -1.953195 -1.423189 -0.434017
H -2.655990 0.222339 -0.246262
H -1.953442 -0.628974 1.184551
C -0.086332 1.490308 0.005539
O 1.107808 1.129995 0.091595
C 0.830850 -0.528023 -0.035191
N 1.358458 -1.572884 0.026174
TS 106
MIN 32 <--> CO+C2H3NO
E= -320.6292957900 ZPE= 32.3967000000
O -0.536397 1.305025 -0.065529
C 2.338638 -0.826400 0.124245
H 2.581601 -1.524508 -0.673653
H 2.912537 -0.848938 1.048371
H -1.769198 0.714886 0.948278
C -1.976173 -0.193331 0.379787
O -1.947804 -1.146026 -0.268019
C 0.702439 1.048146 -0.242409
N 1.394177 0.030869 -0.032050
TS 107
MIN 4 <--> CH2O+C2HNO
E= -320.6256048400 ZPE= 31.8279000000
O 0.715215 -1.192525 0.000084
C 1.844088 -0.592436 -0.000045
H 2.438903 -0.576146 0.934536
H 1.464708 0.661498 -0.000118
H 2.438772 -0.576304 -0.934714
C -0.602378 1.134708 0.000050

O 0.516552 1.579266 -0.000010
C -1.308178 -0.074188 0.000002
N -2.256815 -0.773068 -0.000047
TS 108
HOCH+C2HNO <--> CH2O+C2HNO
E= -320.6242653200 ZPE= 31.1385600000
O 1.418190 -0.851616 0.384074
C 2.250173 -0.282566 -0.449425
H 1.890711 0.694458 -0.849024
H 2.405696 -1.408670 0.142666
H -0.396483 0.760930 1.587154
C -0.550218 0.757301 0.497917
O -0.013248 1.550237 -0.253779
C -1.521417 -0.236815 0.019075
N -2.315813 -1.009030 -0.332652
TS 109
MIN 17 <--> MIN 18
E= -320.6256815600 ZPE= 32.7082100000
O 0.786517 0.066858 -0.700156
C 2.532038 -0.605924 0.382883
H 2.003337 -0.898829 1.313292
H 1.505407 0.740511 -0.642393
H 2.619072 -1.555388 -0.180637
C -0.328751 0.521003 -0.082897
O -0.503785 1.634053 0.327891
C -2.123709 -1.310231 0.111391
N -1.266735 -0.503239 0.002799
TS 110
CH2O+C2HNO <--> CH2+C2HNO2
E= -320.6275394100 ZPE= 34.4414200000
O 0.847979 -0.706263 0.058879
C 2.311087 -0.572978 0.063406
H 2.528687 0.255284 0.734156
H 2.641147 -0.393158 -0.963041
H 0.550374 -1.552364 -0.310641
C -0.204518 0.475347 -0.076807
O 0.228980 1.579753 -0.021439
C -1.530271 -0.050141 0.055834
N -2.541953 -0.630150 -0.002084
TS 111
MIN 44 <--> CH2O+C2HNO
E= -320.6252922400 ZPE= 33.6848500000
O 0.811330 -0.776892 0.180723
C 2.026498 -0.556871 -0.185272
H 2.333245 0.452655 -0.430674
H 2.665244 -1.429938 -0.183380
H 0.122520 1.219839 1.047104
C -0.091817 0.280266 0.289181
O 0.383585 1.501999 -0.158748
C -1.423931 -0.172282 -0.004854
N -2.534975 -0.478583 -0.171883
TS 112
CH2O+C2HNO <--> HNC+CH2O+CO
E= -320.6180766700 ZPE= 29.6889600000
O 1.208969 1.269773 -0.320677
C -2.285636 -0.543167 0.062759

H 1.509449 0.270145 -0.622688
H -3.347988 -0.738564 -0.175251
H -1.744514 -1.316166 0.637271
C 0.603085 1.112282 0.722869
O -1.739553 0.478796 -0.296865
C 1.048003 -1.002055 0.532876
N 1.662145 -1.372332 -0.401432
TS 113
MIN 35 <--> CH2+C2HNO2
E= -320.6223307600 ZPE= 32.6546300000
O -0.404961 1.646782 0.244993
C 2.471095 -0.793701 0.398225
H 0.821138 -0.972507 -0.753714
H 2.284624 -0.231932 1.336179
H 3.212319 -0.165726 -0.133343
C -0.299679 0.508660 -0.103059
O 0.813571 0.007781 -0.690505
C -2.236108 -1.171632 0.188179
N -1.314115 -0.446615 0.030701
TS 114
CO+C2H3NO <--> H2+C3HNO2
E= -320.6153960700 ZPE= 28.3346500000
O -1.180839 0.527155 -0.578609
C -0.401085 1.280202 0.288320
H -1.654111 2.615164 0.790623
H -0.023724 2.080658 -0.372028
H -1.258546 2.026468 1.195438
C 2.433076 -0.047919 -0.319199
O 3.298764 -0.539307 0.229414
C -1.729437 -0.555333 -0.087322
N -2.260336 -1.526681 0.269820
TS 115
CH2O+C2HNO <--> H2+C3HNO2
E= -320.6187456100 ZPE= 30.7637700000
O -1.066463 -0.334629 -0.517607
C -1.979405 -0.777243 0.230173
H -0.404454 0.036642 1.676819
H -1.149632 -0.330772 1.585703
H -2.709058 -1.329679 -0.392920
C 0.101778 0.540382 0.075033
O 0.031765 1.726646 -0.051562
C 1.309581 -0.277459 -0.009909
N 2.278428 -0.918057 -0.012576
TS 116
MIN 17 <--> H2+C3HNO2
E= -320.6164778700 ZPE= 30.3552400000
O -0.726854 -0.711460 0.113566
C -1.984934 -0.507938 -0.371112
H -2.904133 0.319575 1.206011
H -2.712248 0.553361 0.467107
H -2.513753 -1.420289 -0.032321
C 0.169772 0.328718 -0.012579
O -0.106907 1.487782 -0.082947
C 2.582043 -0.548944 0.039083
N 1.456991 -0.184892 0.025986
TS 117

MIN 25 <--> MIN 42
E= -320.6237893900 ZPE= 35.1323400000
O 1.027083 1.339597 0.150199
C -1.711253 0.012603 -0.650373
H 1.386448 1.721247 -0.670895
H -2.148564 -0.834982 -1.169037
H -2.121344 1.003387 -0.815841
C -0.425530 -0.125613 -0.005034
O -1.411671 -0.274982 0.816161
C 0.992889 -0.291260 -0.014602
N 1.831933 -1.140136 -0.150722
TS 118
MIN 17 <--> H2+C3HNO2
E= -320.6159603700 ZPE= 30.3514000000
O -0.136297 1.477473 -0.028541
C -2.037970 -0.565644 -0.302425
H -2.676200 0.128075 1.458046
H -2.790967 -0.543232 1.044297
H -2.177493 0.498890 -0.584367
C 0.166697 0.321471 -0.023402
O -0.715458 -0.756336 -0.052894
C 2.578673 -0.542004 0.079069
N 1.459187 -0.162252 0.030579
TS 119
H2+CO+C2HNO <--> CO+C2H3NO
E= -320.6118838400 ZPE= 27.8943100000
O 1.769392 -0.170935 -0.509386
C 1.961729 -1.272214 0.301309
H 0.933521 -2.324607 -0.093118
H 0.195194 -2.148444 0.157656
H 1.571564 -1.007463 1.306757
C -3.322187 0.122040 -0.028399
O -2.412988 -0.562381 -0.032820
C 1.120421 0.886865 -0.080088
N 0.555530 1.846700 0.258489
TS 120
H2+C3HNO2 <--> CO+C2H3NO
E= -320.6113703900 ZPE= 27.8525600000
O -1.285534 -0.539038 -0.279691
C -0.279917 -0.186345 0.596009
H -0.746528 0.422974 1.398826
H 0.204083 1.609478 -0.096088
H 0.566214 0.898227 -0.076699
C 4.054582 -0.495825 0.042482
O 3.478971 0.456439 -0.194508
C -2.505044 -0.069932 -0.142427
N -3.598427 0.320389 -0.058405
TS 121
MIN 55 <--> MIN 55
E= -320.6226468100 ZPE= 35.4856100000
O 0.890266 -0.268195 0.000008
C 2.331293 -0.473112 -0.000004
H 2.759663 -0.026240 0.897451
H 2.759579 -0.026626 -0.897691
H 2.466528 -1.553230 0.000217
C 0.491512 0.964689 0.000005

O -0.848870 1.026070 -0.000003
C -2.367040 -1.043411 0.000004
N -1.578790 -0.163701 -0.000007
TS 122
H2+C3HNO2 <--> H2+C3HNO2
E= -320.6066908600 ZPE= 26.0832300000
O 1.876154 -0.160320 -0.732263
C 1.012486 -0.153209 0.226692
H 3.624217 -1.523984 1.513825
H 2.174872 -0.624265 0.336994
H 4.017074 -1.458415 0.883415
C -0.331755 0.497921 0.092812
O -0.450697 1.705925 0.175127
C -1.475302 -0.424238 0.039100
N -2.350341 -1.183003 -0.061253
TS 123
MIN 4 <--> CH2+C2HNO2
E= -320.6163363400 ZPE= 32.2474200000
O -0.186787 1.484692 -0.011652
C -2.364644 -0.356867 0.292922
H -2.779574 -1.306741 -0.054808
H -2.527133 0.547638 -0.299827
H -1.494095 -0.647523 -0.882530
C 0.142972 0.328534 -0.030717
O -0.726733 -0.732067 -0.100677
C 1.513085 -0.159030 0.018723
N 2.622925 -0.498599 0.064319
TS 124
MIN 24 <--> H2+C3HNO2
E= -320.6141909100 ZPE= 31.3788500000
O 1.015985 -0.630285 0.830850
C 1.246246 -0.760138 -0.518586
H 1.143351 -1.788845 -1.122452
H 1.373846 1.701925 -0.443409
H 0.205453 -1.867636 -0.955951
C 0.230659 0.211133 -0.071088
O 0.484789 1.551952 -0.086995
C -1.199087 -0.056895 -0.013888
N -2.342250 -0.254769 0.027479
TS 125
MIN 55 <--> CN+C2H3O2
E= -320.6183370700 ZPE= 34.8037500000
O -0.965411 -0.290517 0.000091
C -2.410506 -0.453773 -0.000050
H -2.665111 -1.020691 0.895623
H -2.664917 -1.020912 -0.895639
H -2.892796 0.523783 -0.000223
C -0.495892 0.913152 -0.000106
O 0.780838 1.004688 -0.000007
C 2.665492 -0.811042 -0.000249
N 1.592121 -0.297938 0.000285
TS 126
CH2O+C2HNO <--> HCN+CH2O+CO
E= -320.6101302500 ZPE= 29.8077900000
O -1.463192 -0.878327 -0.115769
C -2.183614 0.092287 0.012169

H -1.770047 1.094501 0.217908
H 1.582491 -0.393386 -0.748706
H -3.281442 -0.004314 -0.080923
C 0.977870 -0.832279 0.708864
O 1.547859 -1.350650 -0.249178
C 1.016978 1.090672 -0.189396
N 0.560609 2.147276 0.048782
TS 127
MIN 20 <--> H2+C3HNO2
E= -320.6106069900 ZPE= 30.1778000000
O -1.039787 0.629658 -0.010534
C -1.869160 -0.390517 -0.329417
H -1.966092 -1.404581 1.360993
H -1.265493 -1.263758 -0.652742
H -2.471780 -0.952085 0.924277
C 0.349566 0.585160 0.012775
O 0.998829 1.582106 0.074480
C 1.484958 -1.724014 -0.014559
N 0.891263 -0.699638 -0.022414
TS 128
MIN 47 <--> CH2O+C2HNO
E= -320.6135214000 ZPE= 33.8241100000
O -2.295903 0.815109 0.056589
C -2.441289 -0.447601 -0.146461
H -1.363387 1.061478 -0.202897
H -3.205987 -0.939820 0.448451
H -1.923808 -0.958483 -0.949284
C 0.987178 -0.773527 0.112194
O -0.092081 -0.173574 0.149826
C 3.238640 0.451487 -0.112001
N 2.127125 0.046055 -0.009997
TS 129
MIN 36 <--> MIN 46
E= -320.6151563400 ZPE= 34.9100700000
O 1.678798 -0.434671 -0.000007
C 2.640312 0.663349 0.000002
H 3.614059 0.176310 -0.000102
H 2.506431 1.265592 0.899198
H 2.506306 1.265726 -0.899084
C 0.414504 -0.095152 0.000002
O -0.481432 -0.893127 0.000004
C -2.327447 -0.061045 0.000002
N -3.224277 0.695978 -0.000003
TS 130
MIN 56 <--> CH2O+C2HNO
E= -320.6140897100 ZPE= 34.9070500000
O -1.684825 -0.611642 -0.166560
C -2.317617 0.627285 0.065041
H -3.317138 0.486410 -0.364704
H -1.816592 1.442733 -0.473991
H -2.408417 0.851474 1.134510
C 0.571508 -0.039348 -0.490621
O -0.194460 -0.450755 0.398630
C 1.926467 0.077212 -0.057087
N 3.070611 0.246811 0.106231
TS 131

CH2O+C2HNO <--> H2+C3HNO2
E= -320.6053331000 ZPE= 30.6137600000
O 2.505038 -0.369977 -0.458656
C 1.788347 0.184347 0.306216
H 1.236643 1.611188 -0.250882
H 1.964885 0.496574 1.342799
H 0.388466 1.557159 -0.423010
C -0.645874 0.400477 -0.148993
O 0.216569 -0.354167 0.375786
C -3.112643 -0.192091 -0.095794
N -1.934547 -0.032596 -0.053502
TS 132
MIN 15 <--> CH2O+C2HNO
E= -320.6061343800 ZPE= 32.8336000000
O 2.175257 0.124041 -0.000003
C 1.358899 -0.958692 0.000001
H 0.952767 -1.356597 0.942545
H 2.461582 -1.354492 0.000000
H 0.952763 -1.356602 -0.942539
C -0.343719 0.291310 0.000002
O 0.263908 1.309542 0.000000
C -1.726206 -0.016175 0.000004
N -2.802040 -0.471376 -0.000004
TS 133
CH2O+C2HNO <--> H2+CO+C2HNO
E= -320.6005221900 ZPE= 29.6058900000
O -1.657019 -0.973006 -0.521170
C -1.219871 -0.381556 0.411028
H -1.743342 0.192139 1.186950
H -0.189843 -1.068140 1.147908
H 0.644733 -1.311793 0.946898
C 1.465823 0.076275 -0.423943
O 1.687748 -0.980281 0.116766
C 0.191469 0.914875 -0.025807
N -0.225986 2.022360 0.026544
TS 134
H2+CO+C2HNO <--> H2+CO+C2HNO
E= -320.5923726200 ZPE= 28.5738700000
O -0.395706 1.387404 0.000000
C -0.677866 0.186747 0.000000
H -0.185145 -0.504588 0.977954
H -0.185145 -0.504588 -0.977955
H 0.138330 -0.778502 0.000000
C 3.448593 0.015701 0.000000
O 2.471086 -0.570348 0.000000
C -3.160550 -0.586564 0.000000
N -2.004592 -0.349154 0.000000
TS 135
MIN 20 <--> MIN 20
E= -320.6016088300 ZPE= 34.6536500000
O -1.451432 -0.251971 0.174954
C -1.337729 1.195926 -0.101535
H -0.512990 1.448889 -0.756322
H -1.235938 1.702271 0.858353
H -2.296448 1.432612 -0.560551
C -0.669512 -1.265576 0.023114

O 0.653757 -1.075766 -0.125406
C 2.219874 0.897231 0.119534
N 1.307283 0.153235 -0.026363
TS 136
 MIN 32 <--> MIN 53
E= -320.5964672700 ZPE= 32.2216200000
O -1.203745 1.191138 -0.214284
C 2.208929 0.534475 0.163888
H 2.891244 0.279350 0.970800
H 2.378502 1.423161 -0.438408
H -2.322262 1.125280 0.275028
C -1.643688 0.074751 0.267989
O -0.916779 -1.034223 0.166971
C 0.375330 -1.059068 -0.430286
N 1.196184 -0.197723 -0.062638
TS 137
 MIN 54 <--> H2+HCO+C2NO
E= -320.5609936300 ZPE= 28.1314500000
O 1.435382 -0.679219 0.018418
C 2.607870 -0.388998 0.165636
H 3.066917 0.260806 0.915754
H 3.234440 0.342320 -1.101538
H 3.389642 -0.543588 -0.800006
C -1.062519 0.983833 -0.020652
O 0.124416 1.096746 0.021265
C -1.918627 -0.150535 -0.011475
N -2.847105 -0.866506 -0.018961
TS 138
 MIN 38 <--> MIN 38
E= -320.5622306600 ZPE= 30.2845800000
O -0.681307 0.393211 -0.018933
C -3.335775 0.307145 0.011657
H -1.759763 0.358244 -0.006505
H -3.975972 0.310862 0.907036
H -3.999785 0.302844 -0.871179
C -0.361884 -0.836931 -0.014263
O 1.037754 -0.989457 0.008305
C 1.826581 0.062375 0.009626
N 2.587202 0.943212 0.001937
TS 139
 MIN 41 <--> MIN 57
E= -320.5613496100 ZPE= 31.7690600000
O -2.639708 -0.651112 -0.220543
C -1.457860 0.762416 0.237378
H -1.475481 1.304322 -0.714161
H -2.557927 0.021344 0.645792
H -2.165728 -1.465046 0.024857
C 0.744428 0.567587 -0.425657
O -0.227242 0.118165 0.356418
C 1.980875 -0.061946 -0.054053
N 3.075725 -0.457912 0.058644
TS 140
 MIN 38 <--> H2+C3HNO2
E= -320.5370958900 ZPE= 29.2254800000
O 0.905174 -0.230147 -0.121372
C 2.260580 -0.401858 -0.340529

H 3.042354 -0.201314 1.076948
H 2.333130 -1.508315 -0.378936
H 2.901186 -0.762094 1.603089
C 0.504783 1.053225 -0.040610
O -0.850110 1.018634 0.050890
C -1.560406 -0.103405 0.040772
N -2.278132 -1.017707 0.043566
TS 141
MIN 38 <--> H2+C3HNO2
E= -320.5368243800 ZPE= 29.0660500000
O -0.905207 -0.288051 -0.116685
C -2.232242 -0.546935 -0.382260
H -3.030771 -0.564434 1.614906
H -2.928993 -1.086832 1.050339
H -2.721334 0.453162 -0.407535
C -0.523957 0.997948 0.010834
O 0.826930 1.008023 0.084814
C 1.580403 -0.084676 0.034742
N 2.337443 -0.965671 0.002480
TS 142
MIN 55 <--> H2+C3HNO2
E= -320.4510156700 ZPE= 27.9067700000
O 0.910311 -0.301776 -0.114019
C 2.242466 -0.531704 -0.371267
H 3.031424 -0.495422 1.595225
H 2.713676 0.475263 -0.418455
H 2.937679 -1.032622 1.037813
C 0.485344 0.965724 0.008073
O -0.825628 1.002310 0.079929
C -2.460284 -0.968929 0.008798
N -1.566485 -0.191719 0.026360
TS 143
H2+CO+C2HNO <--> H2+CN+C2HO2
E= -320.4448538900 ZPE= 27.2869600000
O 1.168822 -0.229430 0.344062
C 1.909528 0.732359 -0.204639
H 0.510135 2.692379 -0.445690
H 0.919959 2.193325 -0.836057
H 2.266228 1.277795 0.694864
C 0.524816 -1.306546 -0.083984
O -0.771425 -1.088109 -0.205251
C -2.075956 1.069609 0.189704
N -1.289405 0.200613 0.009987

The following structures are re-optimized at the MP2/6-311+G(2d,2p) level of theory. ZPE is given in kcal/mol and is calculated at this level. They are selected after a preliminary KMC calculation, and are employed in the second KMC simulation.

The geometry is in Å, the energy (given in a.u.) is a CCSD(T)/6-311+G(3df,2p) single point calculation at the MP2/6-311+G(2d,2p) optimized geometry

The frequencies are given in $cm^{-1}$.

```
TS 12
 MIN 4 <--> MIN 17
E= -320.72878370  ZPE= 36.57607
O         0.060266    1.453992   -0.023145
C        -2.032463   -0.263864   -0.017686
H        -2.194993    0.309319   -0.922617
H        -2.615847   -1.172585   -0.017957
H        -2.246689    0.340630    0.855466
C         0.208725    0.280075    0.038785
O        -0.647840   -0.714355    0.029606
C         1.734048   -0.383557    0.636322
N         1.756609   -0.455769   -0.558729
Freqs: 142,  168,  251,  269,  397,  444,  633,  785,  959,
1152, 1188, 1234, 1492, 1518, 1522, 1870, 1968, 3118, 3219, 3254
TS 13
 MIN 9 <--> MIN 20
E= -320.72587191  ZPE= 36.61217
O       -0.708684   -0.871678   -0.020476
C       -1.848910    0.027619    0.006896
H       -1.831015    0.664211   -0.867239
H       -1.826270    0.616638    0.914319
H       -2.699258   -0.639130   -0.007270
C        0.521315   -0.451001    0.020250
O        1.536019   -1.041943   -0.006082
C        0.596508    1.303428    0.644877
N        0.589198    1.340996   -0.551355
Freqs: 137,  226,  253,  303,  376,  461,  602,  610,  951,
1182, 1190, 1238, 1503, 1521, 1525, 1950, 1966, 3126, 3240, 3250
TS 37
 MIN 9 <--> HCN+CH2O+CO
E= -320.67989524  ZPE= 32.80925
O       1.585518   -0.071785    0.000000
C       1.390487   -1.336355    0.000000
H       1.467408   -1.883321    0.939178
H       1.467408   -1.883321   -0.939178
H      -0.177804   -1.332966    0.000000
C       0.000000    0.872445    0.000000
O      -0.157353    2.007312    0.000000
C      -1.096190   -0.600678    0.000000
N      -2.278303   -0.571012    0.000000
Freqs: 130,  167,  168,  271,  368,  481,  539,  570,  648,
832, 1010, 1210, 1234, 1376, 1553, 1828, 2080, 2267, 3052, 3164
TS 41
 MIN 9 <--> CO+C2H3NO
E= -320.68022217  ZPE= 35.18175
O        -0.701508   -0.502143   -0.569797
C        -1.831906   -0.756955    0.288903
H        -1.518803   -0.847606    1.328714
H        -2.286910   -1.684118   -0.040121
H        -2.539663    0.060558    0.196226
C         1.146100   -0.169805   -0.054762
O         2.015272   -0.872807    0.184835
C         0.115304    0.853245   -0.136238
N        -0.105961    1.987408    0.143922
```

Freqs: 55, 99, 177, 213, 253, 467, 579, 607, 728,
993, 1168, 1174, 1472, 1510, 1524, 2010, 2151, 3067, 3162, 3200
TS 58
MIN 9 <--> CO2+C2H3N
E= -320.66670515 ZPE= 34.24818
O 0.442293 1.252372 0.000020
C -1.870331 0.821116 -0.000016
H -1.604516 1.308230 -0.920127
H -1.604552 1.308218 0.920111
H -2.638115 0.070700 -0.000036
C 0.994439 0.108606 0.000002
O 2.137109 -0.299548 -0.000015
C -0.185178 -0.896199 0.000004
N -1.203088 -1.501554 0.000010
Freqs: 43, 141, 178, 216, 360, 438, 588, 666, 685, 753,
756, 1213, 1253, 1447, 1472, 1789, 2022, 3180, 3379, 3379
TS 60
MIN 20 <--> HNC+CH2O+CO (Note that the IRCs computed with dft
and mp2 differ in the products obtained from this ts. See above)
E= -320.63489128 ZPE= 32.32803
O -1.140644 -0.668769 0.000000
C -0.411580 -1.782478 0.000000
H -0.299572 -2.282375 0.951317
H 0.995908 -0.920179 0.000000
H -0.299574 -2.282377 -0.951315
C -0.680280 0.709445 0.000000
O -1.328546 1.676169 0.000000
C 2.531816 0.639394 0.000000
N 1.531003 0.003939 0.000000
Freqs: 105, 127, 131, 202, 299, 346, 545, 553, 622,
768, 890, 1108, 1195, 1283, 1518, 1885, 1979, 2631, 3142, 3287
TS 67
MIN 9 <--> CO2+C2H3N
E= -320.66070532 ZPE= 35.08422
O -2.155676 0.205106 0.000002
C 1.912813 -0.758517 0.000003
H 1.440129 -0.589486 -0.938735
H 1.440020 -0.589478 0.938680
H 2.901734 -1.208368 0.000057
C -0.986674 -0.124215 -0.000002
O -0.393953 -1.250111 -0.000004
C 0.105341 0.992532 0.000004
N 1.203753 1.441223 -0.000002
Freqs: 98, 254, 282, 290, 450, 498, 612, 660, 711, 739,
762, 1187, 1226, 1469, 1523, 1777, 1998, 3145, 3367, 3495
TS 69
MIN 20 <--> CO2+C2H3N
E= -320.66040012 ZPE= 33.74517
O -0.293987 -1.222345 -0.100229
C 1.771403 -0.911929 0.052115
H 1.958832 -0.387904 0.972373
H 2.031031 -0.403601 -0.861158
H 1.628739 -1.977116 0.053743
C -1.149257 -0.398641 -0.019778
O -2.080605 0.280477 0.051355
C 0.789905 1.506153 -0.630294

```
N        0.700832    1.304295    0.544826
Freqs: 57,  131,  164,  178,  188,  226,  384,  593,  632,  675,
725, 1239, 1341, 1450, 1461, 1926, 2359, 3156, 3353, 3366
TS 144
 MIN 4 <--> MIN 9
E= -320.78860698  ZPE= 37.33329
O        -0.959345   -0.165398    0.656624
C        -1.775674   -0.828227   -0.338194
H        -2.535251   -1.359924    0.216787
H        -1.174958   -1.530983   -0.910994
H        -2.231061   -0.090789   -0.991950
C         0.063186    0.545132    0.120177
O         0.009278    1.697408   -0.215743
C         1.302668   -0.244415    0.018517
N         2.285818   -0.872760   -0.091986
Freqs: 158,  180,  217,  298,  526,  593,  760,  816, 1017,
1171, 1181, 1228, 1499, 1525, 1531, 1762, 2153, 3087, 3178, 3235
TS 145
 MIN 17 <--> MIN 20
E= -320.76469784  ZPE= 37.18011
O       -0.918112   -0.135570    0.656698
C       -1.776548   -0.744866   -0.338393
H       -2.569689   -1.222161    0.218726
H       -1.220500   -1.486806   -0.905687
H       -2.181066    0.020398   -0.993430
C        0.124293    0.527306    0.120955
O        0.148697    1.672065   -0.217628
C        2.196419   -1.025227   -0.117721
N        1.265942   -0.306665    0.025542
Freqs: 127,  146,  176,  258,  544,  589,  774,  834, 1018,
1159, 1182, 1227, 1499, 1525, 1531, 1816, 2089, 3091, 3183, 3238
```

# Kinetic calculations

The kinetic calculations consist of RRKM[4] and KMC[5, 6] calculations. The RRKM rate coefficients for a given process *i* are computed according to the following expression:

$$k_i(E) = \sigma_i \frac{W_i^{TS}(E)}{h\rho_i(E)}$$

where $\sigma_i$ is the reaction path degeneracy, $W_i^{TS}(E)$ is the sum of states at the TS, $\rho_i(E)$ is the density of states at the reactant, and $E$ is the excitation (vibrational) energy of the system. The degeneracy of the reaction path is calculated as $\sigma_i = \frac{m_i^{TS}}{m_i}$, where $m_i$ and $m_i^{TS}$ are the number of optical isomers of the reactant and transition states, respectively. It is generated automatically thanks to a recently developed algorithm that detects symmetry elements from the molecular geometry.[7] The sums and densities of states were evaluated by direct count of the harmonic vibrational states using the Beyer-Swinehart algorithm.[4] An excitation energy $E$ of 148.12 kcal/mol, which corresponds to the laser wavelengths of 193, is employed for the kinetic calculations.

The RRKM rate coefficients computed as detailed above were subsequently employed in two different sets of KMC simulations to follow the transient behavior of the various molecular species that participate in the fragmentation of propenal at 148.12 kcal/mol (193 nm).

**Preliminary KMC simulation**

We first performed a preliminary simulation with all the reactive pathways presenting barrier heights lower than 148.12 kcal/mol (see the table below). For this first simulation, B3LYP/6-31+G(d,p) vibrational frequencies and geometries are employed. To make the KMC simulation simpler, we assume that the conformational isomers form a

microcanonical ensemble and are, therefore, in equilibrium.[8] Thus, the total sum of states of minimum MIN$x$ $\rho_{MINx}(E)$ can be expressed as:

$$\rho_{MINx}(E) = \sum_{j=a}^{N} \rho_{MINxj}(E)$$

Where $N$ is the number of conformational isomers of MIN$x$ and $\rho_{MINxj}(E)$ is the density of states of conformer $j$.

To simplify even more the calculation, all conformers of a given minimum are considered degenerate, and their vibrational frequencies equal to those of the most stable one (denoted as above with the letter a). These two approximations are quite reasonable taken into account the small energy differences of the conformational isomers (see above) and their similar vibrational frequencies.

With this approach, the density of states of a given minimum can be simply computed as $\rho_{MINx}(E) = N\rho_{MINxa}(E)$.

A total of 92 elementary processes are considered in the first (preliminary) simulation, including 42 isomerizations, and the 50 pathways corresponding to the 11 different product channels gathered in Table 3S.

**Table 3S:** Elimination pathways considered in the first KMC simulation.

| Channel | Reactant(s)[a] | Products | Total number of pathways |
|---|---|---|---|
| **(3) $CH_2O$** | 4 (1), 11 (2), 33 (1), 39 (2), 44 (2), 47 (1), 51 (1) | $CH_2O + C_2HNO$ | 10 |
| **(5) CO** | 1 (1), 4 (1), 12 (1), 29 (1), 32 (1), 36 (3), 51 (1) | $CO + C_2H_3NO$ | 9 |
| **(7) $H_2$** | 4 (4), 17 (3), 24 (1) | $H_2 + C_3HNO_2$ | 8 |
| **(6) $CO_2$** | 4 (2), 16 (1), 17 (2), 27 (1) | $CO_2 + C_2H_3N$ | 6 |
| **(12) Triple 1** | 4 (1), 17 (1), 39 (2), 47 (1) | HCN(HNC) + $CH_2O$ + CO | 5 |
| **(10) HOCN** | 2 (1), 7 (1), 11 (1), 23 (1) | HOCN + $C_2H_2O$ | 4 |
| **(2) $CH_2$** | 4 (1), 26 (1), 35 (1) | $CH_2 + C_2HNO_2$ | 3 |
| **(8) HCN(HNC)** | 12 (1), 10 (1) | HCN(HNC) + $C_2H_2O_2$ | 2 |
| **(9) HNCO** | 7 | HNCO + $C_2H_2O$ | 1 |
| **(4) CN** | 55 | $CN + C_2H_3O_2$ | 1 |
| **(13)Triple 2** | 54 | $H_2$ + HCO + NCCO | 1 |

[a]Number of the starting minimum, and the number in parenthesis indicates the number of pathways starting from this minimum.

As seen in Figure 4S, the most important pathways involved in the fragmentation dynamics of MCF at 148.12 kcal/mol are: HNC+$CH_2$+$CO_2$ (49.1%), $CO_2$ + $C_2H_3N$ (30.3%), CO + $C_2H_3NO$ (12.3%), and HCN + $CH_2O$ + CO (7.0%). Minor channels are: $CH_2O$ + $C_2HNO$ (0.5%), $H_2$ + $C_3HNO_2$ (0.4%), and $CH_2$ + $C_2HNO_2$ (0.4%).

Additionally, besides MCF, the other important minimum is MIN17.

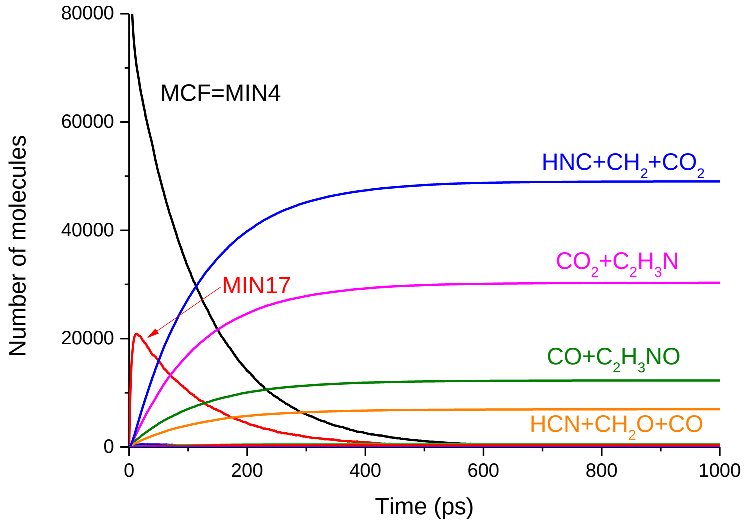


**Figure 4S.** Population of the different species involved in the 148.12 kcal/mol decomposition of MCF, obtained in the preliminary KMC simulation.

**Second KMC simulation**

Then, in a second simulation only the most relevant pathways are included (those with yields greater than 1%, see above), but in this case, MP2/6-311+G(2d,2p) vibrational frequencies and geometries are employed in the simulation. In both cases, CCSD(T)/6-311+G(3df,2p) single point calculations are employed to calculate the barrier heights.

Also, conformational isomers of the most relevant minima (MIN4 and MIN17) are included here (MIN9, which is a conformer of MIN4, as well as MIN20, which is a conformer of MIN17).

The rate coefficients for the 14 relevant elementary steps are collected in Table 4S.

**Table 4S:** Rate coefficients considered in second KMC simulation

| $k(E)(ps^{-1})$ | Reactant | Product(s) | Transition state |
|---|---|---|---|
| 0.07296 | MIN 4 | MIN 17 | TS 12 |
| 0.20432 | MIN 17 | MIN 4 | TS 12 |
| 0.05056 | MIN 9 | MIN 20 | TS 13 |
| 0.18321 | MIN 20 | MIN 9 | TS 13 |
| 0.002484 | MIN 9 | $HCN + CH_2O + CO$ | TS 37 |
| 0.009504 | MIN 9 | $CO + C_2H_3NO$ | TS 41 |
| 0.001278 | MIN 9 | $CO_2 + C_2H_3N$ | TS 58 |
| 0.00006268 | MIN 20 | $HNC + CH_2O + CO$ | TS 60 |
| 0.00004063 | MIN 9 | $CO_2 + C_2H_3N$ | TS 67 |
| 0.025260 | MIN 20 | $CO_2 + C_2H_3N$ | TS 69 |
| 3.989 | MIN 4 | MIN 9 | TS 144 |
| 4.398 | MIN 9 | MIN 4 | TS 144 |
| 3.572 | MIN 17 | MIN 20 | TS 145 |
| 4.915 | MIN 20 | MIN 17 | TS 145 |

The most important difference between the MP2/6-311+G(2d,2p) and the B3LYP/6-31+G(d,p) optimizations regards TS60. First of all, the B3LYP/6-31+G(d,p) frequencies of this structure are (in $cm^{-1}$):

42, 81, 123, 139, 174, 301, 338, 625, 625, 867, 900, 1114, 1338, 1340, 1410, 1448, 2199, 2404, 3063, 3157

On the other hand, the MP2/6-311+G(2d,2p) frequencies are (in $cm^{-1}$):

105, 127, 131, 202, 299, 346, 545, 553, 622, 768, 890, 1108, 1195, 1283, 1518, 1885, 1979, 2631, 3142, 3287.

Thus, the MP2 transition state is much tighter than the B3LYP one. Additionally, the energy of the MP2 geometry is much higher:

$E_{TS60,\ CCSD(T)/6\text{-}311+G(3df,2p)//MP2/6\text{-}311+G(2d,2p)}$ = 103.0 kcal/mol

$E_{TS60,CCSD(T)/6\text{-}311+G(3df,2p)//B3LYP/6\text{-}31+G(d,p)}$ = 86.4 kcal/mol

Finally, the MP2 IRC from TS60 leads to HNC+$CH_2O$+CO, while the B3LYP one leads to HNC+$CH_2$+$CO_2$

As a consequence of this, the HNC+$CH_2O$+CO pathway has a negligible contribution (its yield is only 0.1%) to the fragmentation dynamics of MCF, when the PES is computed with the higher levels of theory. The second KMC simulation provides the following product yields:

| | |
|---|---|
| CO + $C_2H_3NO$ | 47% |
| $CO_2$ + $C_2H_3N$ | 40% |
| HCN + $CH_2O$ + CO | 13% |

# QCT simulations

## PM3-SRP

For the QCT simulations a PM3 with Specific Reaction Parameters[9] (PM3-SRP) Hamiltonian is employed. The parametrization has been carried out using a genetic algorithm developed by Marques and co-workers[10, 11] and recently implemented in a multipurpose optimization program.[12] The MP2/6-311+G(2d,2p) vibrational frequency calculations and the single point CCSD(T)/6-311+G(3df,2p) results are employed as the benchmark. Tables 5S and 6S collect the features of the PESs considered in the parametrization (geometries, vibrational frequencies and energies), corresponding to the HCN and HNC elimination channels, respectively.

**Table 5S:** PES features considered in the reparametrization of the PM3 Hamiltonian for the HCN elimination channel via TS37.

| TS 37[a] | Ab initio[b] | PM3 | PM3-SRP |
|---|---|---|---|
| $r_{12}$ | 1.28 | 1.31 | 1.19 |
| $r_{13}$ | 2.04 | 2.02 | 1.95 |
| $r_{14}$ | 2.04 | 2.02 | 1.95 |
| $r_{15}$ | 2.17 | 2.18 | 2.14 |
| $r_{16}$ | 1.84 | 1.42 | 1.85 |
| $r_{17}$ | 2.71 | 2.32 | 2.66 |
| $r_{18}$ | 2.73 | 2.71 | 2.61 |
| $r_{19}$ | 3.90 | 3.81 | 3.84 |
| $r_{23}$ | 1.09 | 1.09 | 1.06 |
| $r_{24}$ | 1.09 | 1.09 | 1.06 |
| $r_{25}$ | 1.57 | 1.56 | 1.65 |
| $r_{26}$ | 2.61 | 2.34 | 2.55 |
| $r_{27}$ | 3.68 | 3.44 | 3.57 |
| $r_{28}$ | 2.59 | 2.60 | 2.61 |
| $r_{29}$ | 3.75 | 3.76 | 3.78 |
| $r_{34}$ | 1.88 | 1.89 | 1.82 |
| $r_{35}$ | 1.97 | 2.08 | 2.05 |
| $r_{36}$ | 3.26 | 3.03 | 3.19 |
| $r_{37}$ | 4.32 | 4.09 | 4.20 |
| $r_{38}$ | 3.02 | 3.14 | 3.07 |
| $r_{39}$ | 4.08 | 4.24 | 4.14 |

| | | | |
|---|---|---|---|
| $r_{45}$ | 1.97 | 2.08 | 2.05 |
| $r_{46}$ | 3.26 | 3.03 | 3.19 |
| $r_{47}$ | 4.32 | 4.09 | 4.20 |
| $r_{48}$ | 3.02 | 3.14 | 3.07 |
| $r_{49}$ | 4.08 | 4.24 | 4.14 |
| $r_{56}$ | 2.21 | 2.22 | 2.06 |
| $r_{57}$ | 3.34 | 3.34 | 3.18 |
| $r_{58}$ | 1.17 | 1.21 | 1.18 |
| $r_{59}$ | 2.23 | 2.31 | 2.20 |
| $r_{67}$ | 1.15 | 1.16 | 1.13 |
| $r_{68}$ | 1.84 | 2.03 | 1.53 |
| $r_{69}$ | 2.70 | 2.87 | 2.51 |
| $r_{78}$ | 2.77 | 2.91 | 2.46 |
| $r_{79}$ | 3.34 | 3.44 | 3.13 |
| $r_{89}$ | 1.18 | 1.17 | 1.23 |
| $\omega_1^{\ddagger}$ | 786i | 858i | 782i |
| $\omega_2^{\ddagger}$ | 130 | 110 | 125 |
| $\omega_3^{\ddagger}$ | 167 | 201 | 164 |
| $\omega_4^{\ddagger}$ | 168 | 201 | 172 |
| $\omega_5^{\ddagger}$ | 271 | 339 | 291 |
| $\omega_6^{\ddagger}$ | 368 | 398 | 381 |
| $\omega_7^{\ddagger}$ | 481 | 421 | 457 |
| $\omega_8^{\ddagger}$ | 539 | 464 | 517 |
| $\omega_9^{\ddagger}$ | 570 | 519 | 560 |
| $\omega_{10}^{\ddagger}$ | 648 | 597 | 628 |
| $\omega_{11}^{\ddagger}$ | 832 | 899 | 827 |
| $\omega_{12}^{\ddagger}$ | 1010 | 904 | 942 |
| $\omega_{13}^{\ddagger}$ | 1210 | 995 | 1208 |
| $\omega_{14}^{\ddagger}$ | 1234 | 1150 | 1212 |
| $\omega_{15}^{\ddagger}$ | 1376 | 1260 | 1397 |
| $\omega_{16}^{\ddagger}$ | 1553 | 1372 | 1553 |
| $\omega_{17}^{\ddagger}$ | 1828 | 1631 | 1834 |
| $\omega_{18}^{\ddagger}$ | 2080 | 2126 | 1954 |
| $\omega_{19}^{\ddagger}$ | 2267 | 2346 | 2260 |
| $\omega_{20}^{\ddagger}$ | 3052 | 3016 | 3176 |
| $\omega_{21}^{\ddagger}$ | 3164 | 3095 | 3191 |
| Products[a] | Ab initio[b] | PM3 | PM3-SRP |
| $r_{12}$ | 1.21 | 1.20 | 1.15 |
| $r_{13}$ | 2.02 | 2.00 | 1.93 |
| $r_{14}$ | 2.02 | 2.00 | 1.93 |
| $r_{23}$ | 1.10 | 1.09 | 1.06 |
| $r_{24}$ | 1.10 | 1.09 | 1.06 |
| $r_{34}$ | 1.87 | 1.85 | 1.82 |
| $r_{67}$ | 1.14 | 1.13 | 1.11 |
| $r_{58}$ | 1.06 | 1.07 | 1.04 |
| $r_{59}$ | 2.23 | 2.23 | 2.22 |

| | | | |
|---|---|---|---|
| $r_{89}$ | 1.17 | 1.16 | 1.18 |
| $\omega_1$ | 715 | 858 | 739 |
| $\omega_2$ | 2015 | 2285 | 2077 |
| $\omega_3$ | 3464 | 3297 | 3453 |
| Reverse barrier height[c] | Ab initio[b] | PM3 | PM3-SRP |
| $\Delta E_r^{\ddagger}$ | 53.1 | 49.9 | 55.2 |

[a]$r$ are distances in Å, $\omega^{\ddagger}$ and $\omega$ are vibrational frequencies in $cm^{-1}$.
[b]MP2/6-311+G(2d,2p) results for geometries and vibrational frequencies and CCSD(T)/6-311+G(3df,2p)//MP2/6-311+G(2d,2p) result for the reverse barrier.
[c]This value is calculated as the energy of the transition state minus the energy of the products (in kcal/mol)

**Table 6S:** PES features considered in the reparametrization of the PM3 Hamiltonian for the HNC elimination channel via TS60.

| TS 60[a] | Ab initio[b] | PM3 | PM3-SRP |
|---|---|---|---|
| $r_{12}$ | 1.33 | 1.32 | 1.38 |
| $r_{13}$ | 2.05 | 2.02 | 1.90 |
| $r_{14}$ | 2.15 | 2.16 | 2.33 |
| $r_{15}$ | 2.05 | 2.02 | 1.90 |
| $r_{16}$ | 1.45 | 1.40 | 1.36 |
| $r_{17}$ | 2.35 | 2.35 | 2.45 |
| $r_{18}$ | 3.90 | 3.78 | 4.07 |
| $r_{19}$ | 2.76 | 2.64 | 2.85 |
| $r_{23}$ | 1.08 | 1.09 | 1.12 |
| $r_{24}$ | 1.65 | 1.61 | 1.61 |
| $r_{25}$ | 1.08 | 1.09 | 1.12 |
| $r_{26}$ | 2.51 | 2.32 | 2.35 |
| $r_{27}$ | 3.58 | 3.45 | 3.52 |
| $r_{28}$ | 3.81 | 3.74 | 3.72 |
| $r_{29}$ | 2.64 | 2.56 | 2.54 |
| $r_{34}$ | 2.11 | 2.17 | 2.39 |
| $r_{35}$ | 1.90 | 1.88 | 1.77 |
| $r_{36}$ | 3.16 | 3.02 | 2.99 |
| $r_{37}$ | 4.20 | 4.10 | 4.11 |
| $r_{38}$ | 4.18 | 4.25 | 4.45 |
| $r_{39}$ | 3.08 | 3.13 | 3.31 |
| $r_{45}$ | 2.11 | 2.17 | 2.43 |
| $r_{46}$ | 2.34 | 2.12 | 2.39 |
| $r_{47}$ | 3.48 | 3.21 | 3.36 |
| $r_{48}$ | 2.19 | 2.20 | 2.14 |
| $r_{49}$ | 1.07 | 1.09 | 1.05 |
| $r_{56}$ | 3.16 | 3.02 | 3.02 |
| $r_{57}$ | 4.20 | 4.10 | 4.16 |
| $r_{58}$ | 4.18 | 4.25 | 4.48 |

| | | | |
|---|---|---|---|
| $r_{59}$ | 3.08 | 3.13 | 3.35 |
| $r_{67}$ | 1.16 | 1.16 | 1.17 |
| $r_{68}$ | 3.21 | 2.83 | 3.40 |
| $r_{69}$ | 2.32 | 1.94 | 2.35 |
| $r_{78}$ | 4.00 | 3.31 | 3.81 |
| $r_{79}$ | 3.31 | 2.76 | 3.03 |
| $r_{89}$ | 1.19 | 1.20 | 1.23 |
| $\omega_1^\ddagger$ | 157i | 833i | 167i |
| $\omega_2^\ddagger$ | 105 | 112 | 106 |
| $\omega_3^\ddagger$ | 127 | 174 | 120 |
| $\omega_4^\ddagger$ | 131 | 191 | 134 |
| $\omega_5^\ddagger$ | 202 | 338 | 184 |
| $\omega_6^\ddagger$ | 299 | 390 | 302 |
| $\omega_7^\ddagger$ | 346 | 403 | 338 |
| $\omega_8^\ddagger$ | 545 | 474 | 452 |
| $\omega_9^\ddagger$ | 553 | 549 | 539 |
| $\omega_{10}^\ddagger$ | 622 | 620 | 625 |
| $\omega_{11}^\ddagger$ | 768 | 885 | 813 |
| $\omega_{12}^\ddagger$ | 890 | 911 | 1098 |
| $\omega_{13}^\ddagger$ | 1108 | 995 | 1204 |
| $\omega_{14}^\ddagger$ | 1195 | 1112 | 1206 |
| $\omega_{15}^\ddagger$ | 1283 | 1218 | 1337 |
| $\omega_{16}^\ddagger$ | 1518 | 1390 | 1508 |
| $\omega_{17}^\ddagger$ | 1885 | 1754 | 2046 |
| $\omega_{18}^\ddagger$ | 1979 | 2117 | 2119 |
| $\omega_{19}^\ddagger$ | 2631 | 2192 | 2554 |
| $\omega_{20}^\ddagger$ | 3142 | 3037 | 2926 |
| $\omega_{21}^\ddagger$ | 3287 | 3109 | 2999 |
| Products[a] | Ab initio[b] | PM3 | PM3-SRP |
| $r_{12}$ | 1.21 | 1.20 | 1.21 |
| $r_{13}$ | 2.02 | 2.00 | 2.04 |
| $r_{14}$ | 2.02 | 2.00 | 2.04 |
| $r_{23}$ | 1.10 | 1.09 | 1.12 |
| $r_{24}$ | 1.10 | 1.09 | 1.12 |
| $r_{34}$ | 1.87 | 1.85 | 1.87 |
| $r_{67}$ | 1.14 | 1.13 | 1.15 |
| $r_{58}$ | 1.00 | 0.98 | 0.97 |
| $r_{59}$ | 2.17 | 2.15 | 2.18 |
| $r_{89}$ | 1.18 | 1.18 | 1.21 |
| $\omega_1$ | 441 | 616 | 437 |
| $\omega_2$ | 2012 | 2168 | 2098 |
| $\omega_3$ | 3826 | 3577 | 3654 |
| Reverse barrier height[c] | Ab initio[b] | PM3 | PM3-SRP |
| $\Delta E_r^\ddagger$ | 66.60 | 59.33 | 66.05 |

[a] $r$ are distances in Å, $\omega^\ddagger$ and $\omega$ are vibrational frequencies in $cm^{-1}$.

[b]MP2/6-311+G(2d,2p) results for geometries and vibrational frequencies and CCSD(T)/6-311+G(3df,2p)//MP2/6-311+G(2d,2p) result for the reverse barrier.
[c]This value is calculated as the energy of the transition state minus the energy of the products (in kcal/mol)

The genetic algorithm minimizes the following function

$$f = \sum_{i} ({X_i}^{ab\ initio} - {X_i}^{PM3-SRP})^2\, w_{X_i}$$

Where $X_i$ is each of the values of the table, and $w$ are the weights given by:

$$w_{X_i} = \frac{100}{(1 + X_i^{ab\ initio})^2}$$

Figures 5S and 6S provide the atom labelling employed in Tables 5S and 6S, respectively.

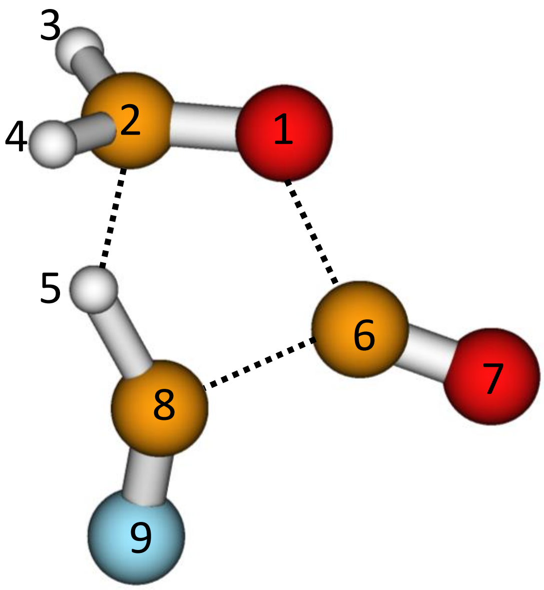


**Figure 5S.** Atomic labelling employed in the definition of the inter-atomic distances of Table 5S.

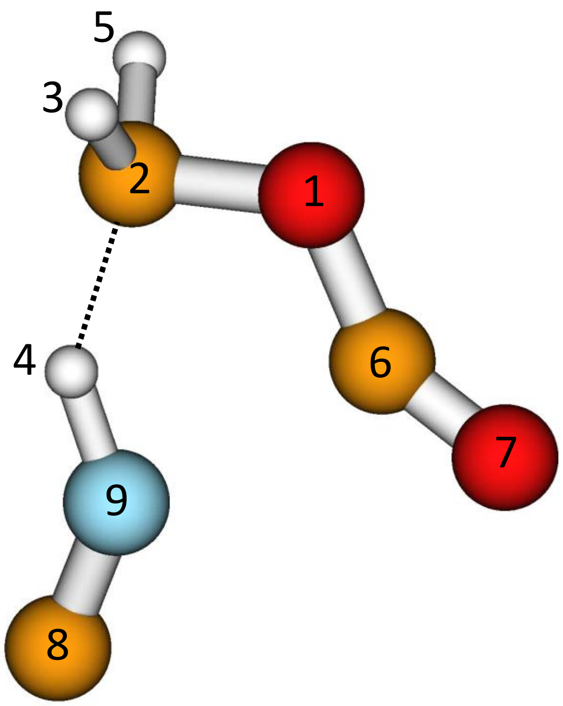


**Figure 6S.** Atomic labelling employed in the definition of the inter-atomic distances of Table 6S.

The optimized parameters of the PM3-SRP Hamiltonians are collected in Tables 7S.

**Table 7S:** Optimized parameters of the PM3-SRP Hamiltonians.

| Parameter | Atom | HCN elimination | HNC elimination |
|---|---|---|---|
| USS | H | -13.973308428950 | -12.289663618909 |
| BETAS | H | -6.131725831385 | -5.957756623585 |
| ZS | H | 1.055506320188 | 1.053183271741 |
| GSS | H | 14.935297423592 | 14.244862122018 |
| USS | C | -46.999583872350 | -49.897995038207 |
| UPP | C | -38.324533056129 | -34.042961082931 |
| BETAS | C | -11.527653889669 | -11.883195334210 |
| BETAP | C | -9.060338037487 | -10.555837431784 |
| ZS | C | 1.554243908158 | 1.474766773849 |
| ZP | C | 1.854922937548 | 1.786235068617 |
| GSS | C | 10.239485710938 | 11.701258049474 |
| GSP | C | 10.696969871595 | 9.416113436775 |
| GPP | C | 11.047527252777 | 11.762052745473 |
| GP2 | C | 9.823023801961 | 9.931583096799 |

| | | | |
|---|---|---|---|
| HSP | C | 2.271176689844 | 2.104837994592 |
| USS | N | -49.289650605585 | -49.974929604105 |
| UPP | N | -42.802053635876 | -50.007404051819 |
| BETAS | N | -12.835227316072 | -14.754967261355 |
| BETAP | N | -18.793109117285 | -20.449557323972 |
| ZS | N | 2.223461452282 | 2.175041485405 |
| ZP | N | 2.535082624010 | 2.121230717162 |
| GSS | N | 10.844283007851 | 11.714641306747 |
| GSP | N | 7.887550592442 | 6.687955261829 |
| GPP | N | 12.790840902433 | 12.241594974944 |
| GP2 | N | 11.670324017791 | 11.411262628940 |
| HSP | N | 1.074946015774 | 1.129373860495 |
| USS | O | -82.137605044574 | -84.821079570274 |
| UPP | O | -75.431152493982 | -66.194371463225 |
| BETAS | O | -43.023610799405 | -45.326959473098 |
| BETAP | O | -26.406210293960 | -22.565772446289 |
| ZS | O | 3.502076009152 | 3.534379349993 |
| ZP | O | 2.500979318568 | 2.269745495124 |
| GSS | O | 16.887659594415 | 16.604719763931 |
| GSP | O | 10.852996814305 | 10.378159185665 |
| GPP | O | 12.673251678445 | 13.278983415122 |
| GP2 | O | 11.810200904730 | 11.530929053610 |
| HSP | O | 0.606927640584 | 0.641389569700 |

**QCT Details**

The general chemical dynamics programs VENUS05[13] has been employed to carry out the simulations. Since the aim is to simulate the HCN and HNC elimination pathways, observed in the 193 nm (148 kcal/mol) photolysis of the molecule, excess vibrational energies of 72.7 and 34.12 kcal/mol are placed at TS 37 and TS 60, respectively, using quasi-classical normal mode sampling[14, 15] and zero rotational energy. Two ensembles of around $8\times10^4$ trajectories are integrated using a sixth-order Adams Moulton predictor-corrector algorithm with fixed time steps of 0.1 fs, which ensured average energy conservations of 99.99%.

The integration finishes when all inter-fragment distances reached at least 15 Å. At this point, the partitioning of the HCN and HNC internal energies are calculated. Additionally,

the rotational quantum numbers $J$ of HCN and HNC are obtained by equating the modulus of the classical rotational angular momentum to $[J(J + 1)]^{1/2}\hbar$. The vibrational states of hydrogen cyanide and hydrogen isocyanide $\mathbf{n}=(n_1 n_2^l n_3)$, where $l$ refers to the vibrational angular momentum, are also calculated here. For the vibrational quantum numbers, the normal mode analysis approach, including anharmonicity and Coriolis coupling terms, of Espinosa-Garcia is employed.[16] The vibrational angular momentum $l$ is computed from $j_a = l\hbar$, where $j_a$ is the projection of the rotational angular momentum of the molecule $j$ onto the molecular axis. The (real) values of the classical actions thus obtained are rounded to the nearest integers to obtain the vibrational states.

The probabilities of the vibrational states are obtained using both the standard histogram binning (HB), and an energy-based Gaussian binning (1GB) procedure.[17-20] More specifically, a noninteger classical harmonic action for each mode is obtained as

$$n'_k = \frac{E_k}{\omega_k} - \frac{1}{2} \quad k = 1,2,3$$

Where $E_k$ and $\omega_k$ are the vibrational energy and frequency for mode $k$, respectively. The integer vibrational quanta are determined by rounding $n_k$' to the nearest integer $n_k$. Additionally, the vibrational quantum number $l$ is determined by rounding $\frac{j_a}{\hbar}$, where $j_a$ is the projection of the rotational angular momentum onto the molecular axis, to the nearest (even or odd) integer. Also, if the value of $l$ thus determined is greater than $n_2$, $l$ is equated to $n_2$.

In the standard histogram binning (HB), the probability of a particular vibrational state $\mathbf{n}$ $(=n_1 n_2^l n_3)$ is:

$$P_{\text{HB}}(\mathbf{n}) = \frac{N(\mathbf{n})}{N_{traj}}$$

Where $N(\mathbf{n})$ is the number of HCN (or HNC) molecules in state $\mathbf{n}$, and $N_{traj}$ the total number of trajectories.

By contrast, in the 1GB approach, a Gaussian weight is employed

$$P_{1\mathrm{GB}}(\mathbf{n}) = \frac{\frac{\beta}{\sqrt{\pi}} \sum_{p=1}^{N(\mathbf{n})} e^{-\beta^2 \{[E(\mathbf{n}_p') - E(\mathbf{n})]/2E(0)\}^2}}{N_{traj}} \qquad p = 1,2,\ldots,N(\mathbf{n})$$

Where $\beta = 2(ln2)^{1/2}/\delta$, $\delta$ is the full-width at half maximum is taken as 0.1, $E(0)$ is the harmonic zero-point energy (ZPE), and

$$E(\mathbf{n}_p{}') = \sum_{k=1}^{3} \omega_k (n_{k,p}' + 1/2)$$

$$E(\mathbf{n}) = \sum_{k=1}^{3} \omega_k (n_k + 1/2)$$

The calculated HCN and HNC vibrational distributions using both HB and 1GB methods are shown in Figure 7S in comparison with the measure nascent distributions.

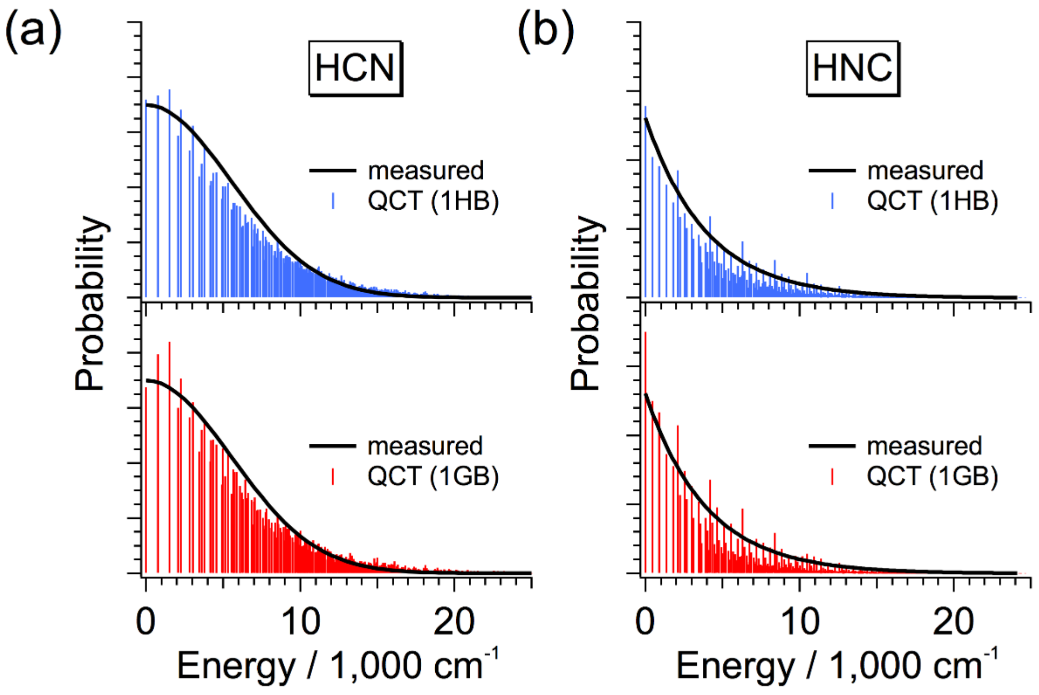

**Figure 7S.** Direct comparison of the measured (black line) and QCT simulated (top blue, bottom red lines) nascent population distributions of (a) HCN and (b) HNC.

## References


1. E. Martínez-Núñez, *J. Comput. Chem.*, 2015, **36**, 222.
2. E. Martínez-Núñez, *Phys. Chem. Chem. Phys.*, 2015, **17**, 14912.
3. J. J. P. Stewart, *J. Mol. Model.*, 2013, **19**, 1.
4. G. Smith and R. G. Gilbert, *Theory of unimolecular and recombination reactions*, Blackwell Scientific Publications, Oxford, 1990.
5. A. B. Bortz, M. H. Kalos and J. L. Lebowitz, *J. Comput. Phys.*, 1975, **17**, 10.
6. D. T. Gillespie, *J. Comput. Phys.*, 1976, **22**, 403.
7. O. Beruski and L. N. Vidal, *J. Comput. Chem.*, 2014, **35**, 290.
8. G. H. Peslherbe and W. L. Hase, *J. Chem. Phys.*, 1994, **101**, 8535.
9. A. Gonzalez-Lafont, T. N. Truong and D. G. Truhlar, *J. Phys. Chem.* , 1991, **95**, 4618.
10. J. M. C. Marques, F. B. Pereira and T. Leitao, *J. Phys. Chem. A*, 2008, **112**, 6079.
11. J. M. C. Marques, F. V. Prudente, F. B. Pereira, M. M. Almeida, A. M. Maniero and C. E. Fellows, *J. Phys. B*, 2008, **41**, 085103.
12. R. Rodriguez-Fernandez, *GAFit: A multipurpose minimization program*, (2014).
13. W. L. Hase, R. J. Duchovic, X. Hu, A. Komornicki, K. F. Lim, D.-H. Lu, G. H. Peslherbe, K. N. Swamy, S. R. Vande Linde, A. Varandas, H. Wang and R. J. Wolf, *Quantum Chemistry Program Exchange (QCPE) Bulletin*, 1996, **16**, 671.
14. K. Bolton, W. L. Hase and G. H. Peslherbe, *Modern Methods for Multidimensional Dynamics Computations in Chemistry*, World Scientific, Singapore, 1998.
15. C. Doubleday Jr, K. Bolton, G. H. Peslherbe and W. L. Hase, *J. Am. Chem. Soc.*, 1996, **118**, 9922.
16. J. C. Corchado and J. Espinosa-Garcia, *Phys. Chem. Chem. Phys.*, 2009, **11**, 10157.
17. G. Czabo, *J. Phys. Chem. A*, 2012, **116**, 7467.
18. G. Czabo and J. M. Bowman, *J. Chem. Phys.*, 2009, **131**, 244302.
19. L. Bonnet and J. C. Rayez, *Chem. Phys. Lett.*, 2004, **397**, 106.
20. L. Bonnet and J. C. Rayez, *Chem. Phys. Lett.*, 1997, **277**, 183.
